# Supplementary material for: Measuring the Validity of Clustering Validation Datasets
Source: arXiv:2503.01097 source file (2025-03-03)
Supplement: Supplementary file 1 [file A_within_dataset_axioms.tex]

% \newpage

\section{Ackerman \& Ben-David's \cite{bendavid08nips} Within-dataset Axioms }

\label{app:within}

\noindent
\textbf{(Axiom W1) \textit{Scale Invariance} } \textit{A measure $f$ satisfies scale invariance if for every clustering $C$ of $(X, d)$, and every positive $\alpha$, $f(C, X, d) = f(C, X, \alpha d)$ (where $\alpha d$ is defined by setting, for every pair of domain points $x, y$, $\alpha d(x,y) = \alpha \cdot d(x,y)$)
}

\noindent
\textbf{$C$-consistent variant (Used in W2)} \textit{Given a clustering $C$ over $(X, d)$, a distance function $d'$ is $C$-consistent variant of $d$, if $d'(x, y) \leq d(x,y)$ for all $x \sim_C y$, and $d'(x, y) \geq d(x,y)$ for all $ x \nsim_C y$.}

\noindent
\textbf{(Axiom W2) \textit{Consistency} } \textit{A measure $f$ satisfies consistency if for every clustering $C$ over $(X, d)$, whenever $d'$ is a $C$-consistent variant of $d$, then   $f(C, X, d') \geq f(C, X, d)$}

% The third axiom requires the measures to be rich; any clustering should have an opportunity to have a best score over the domain by modifying the distance function. 
\noindent
\textbf{(Axiom W3) \textit{Richness}} \textit{A measure $f$ satisfies richness if
for each non-trivial clustering $C$ of $X$, there exists a distance function $d$ over $X$ such that $X = \arg\max f(C_i, X, d)$.}

% The last axiom is added to prevent a function that consider the identity of domain points (e.g., relate class labels to the score) to be regarded as a within-dataset internal measure.
\noindent
\textbf{Clustering Isomorphism (Used in W4)} \textit{Two clustering $C$ and $C'$ over the same domain, $(X, d)$, are isomorphic, denoted $C \approx_d C' $, if there exists a distance-preserving isomorphism $\phi: X \rightarrow X$, such that for all $ x, y \in X$, $x \sim_C y$ if and only if $\phi(x) \sim_{C'} \phi(y)$.}

\noindent
\textbf{(Axiom W4) \textit{Isomorphism Invariance}} \textit{A measure $f$ is isomorphism invariant if for all clusterings $C, C'$ over $(X, d)$ where $C \approx_d C'$, $f(C, X, d) = f(C', X, d)$}
