# Supplementary material for: Measuring the Validity of Clustering Validation Datasets
Source: arXiv:2503.01097 source file (2025-03-03)
Supplement: Supplementary file 2 [file C_generalization.tex]

\section{Generalization of Remaining IVMs}

\label{app:gener}

Here, we describe the adjustment process of the remaining IVMs, which we explain briefly in \autoref{sec:remaining}.

\subsection{Adjusting the Dunn Index ($DI$)}

Dunn Index \cite{dunn74joc} is defined as:
\[
DI(C, X, d) = \frac{\displaystyle \min_{1 \leq i \leq |C|} \min_{1 \leq j \leq |C|} \min_{x \in C_i, y \in C_j} d(x,y)}{\displaystyle \max_{1 \leq k \leq |C|} \max_{x, y \in C_k} d(x,y)}.
\]
$DI$ satisfies none of the across-dataset axioms; thus we applied every possible protocols we provided (\autoref{sec:tricks}). 

\noindent
\textbf{Applying T1 (Data-cardinality invariance)} Both the denominator (maximum intra-class distance) and numerator (minimum inter-class distance) of $DI$ compute the minimum or maximum over point pairwise distances, which is very sensitive to noise. We thus first change the denominator and numerator into the maximum average intra-class distance and minimum average inter-class distance, respectively, leading to:
\[
DI_1(C, X, d) = \frac{\displaystyle \min_{1 \leq i \leq |C|} \min_{1 \leq j \leq |C|} \frac{\sum_{x \in C_i, y \in C_j} d(x,y)}{|C_i| \cdot |C_j|}}{\displaystyle \max_{1 \leq k \leq |C|} \frac{\sum_{x, y \in C_k} d(x,y)}{(k \cdot (k - 1)) / 2}}.
\]

\noindent
\textbf{Applying T2 (Shift invariance)} As both denominator and numerator of $DI_1$ consist of type-1 distances, we can directly apply the exponential protocol, hence:
% \[
% DI_2(C, X, d) = \frac{(e^{\min_{1 \leq i \leq |C|} (\min_{1 \leq j \leq |C|} \frac{\sum_{x \in C_i, y \in C_j} d(x,y)}{|C_i| \cdot |C_j|})})^{1/\sigma_d}}{(e^{\max_{1 \leq k \leq |C|} \frac{\sum_{x, y \in C_k} d(x,y)}{(k \cdot (k - 1)) / 2}})^{(1 / \sigma_d)}},
% \]

\[
DI_2(C, X, d) = \frac{\displaystyle \exp\left(\frac{1}{\sigma_d}\min_{1 \leq i \leq |C|} \min_{1 \leq j \leq |C|} \frac{\displaystyle\sum_{x \in C_i, y \in C_j} d(x,y)}{|C_i| \cdot |C_j|}\right)}{\displaystyle \exp\left(\frac{1}{\sigma_d}\max_{1 \leq k \leq |C|} \frac{\displaystyle \sum_{x, y \in C_k} d(x,y)}{(k \cdot (k - 1)) / 2}\right)},
\]
where $\sigma_d = \text{std}(\{d(x,c)| x \in X\})$.

\noindent
\textbf{Applying T4 (Range invariance)}
In the case of maximum score, as $\max(DI_2) \rightarrow + \infty$, we apply the logistic function (T4-b), resulting in $DI_3 = 1/(1+ e^{-k \cdot DI_2})$, to achieve $DI_{3\max} \rightarrow 1$. As we did for $CH$, we estimate the worst score as the expectation of $DI_3$ over random clustering partitions $C^\pi$ (T4-a): $DI_{3\min} = E_\pi (DI_3(C^\pi, X, d))$. We then get $DI_4 = (DI_3 - DI_{3\min}) / (DI_{3\max} - DI_{3\min})$. We set the growth rate $k$ by calibrating $DI_4$ using human-judgement separability scores (T4-c).

\noindent
\textbf{Applying T3 (class-cardinality invariance)} As in $CH_A$ (\autoref{sec:gener}), we make $DI_A$ class-cardinality invariant by averaging class-pairwise scores:
\[
DI_A = \frac{1}{{|C| \choose 2}} \sum_{S \subseteq C, |S|=2} DI_4(C, X, d).
\]

\noindent\sloppy
\textbf{Approaching $DI_{3}$'s minimum bound}
We found that $DI_{3\min}$ can get closer to the minimum bound of $DI_{3}$ by defining $DI_{3\min} = DI_3(C^{\psi}, X, d)$; $C^{\psi} = \{C^{\psi}_1, C^{\psi}_2\}$ satisfying $|C^{\psi}_1| = \{x\}$ and $|C^{\psi}_2| = X \setminus \{x\}$ where $x$ is the geometric median of $X$ (i.e., $x = \arg\min_{x' \in  X} \sum_{y\in X} d(x',y)$). $DI_3(C^{\psi}, X, d)$  is always smaller than $DI_3(C^{\pi}, X, d)$, thus always closer to the worst case (Proof in \autorefapp{app:proofs}). 

\fussy

\noindent
\textbf{Computational Complexity}
The computational complexity of $DI$, $DI_1$, $DI_2$, $DI_3$ is $O(|X|^2\Delta_X)$. 
If we use the geometric median-based worst-case approximation, the performance of $DI_{3\min}$ also depends on the time complexity of the algorithm that computes the geometric median. We use the one proposed by Vardi and Zhang \cite{vardi00nas}; the complexity is $O(|X|\Delta_X \tau)$ where $\tau$ is the number of iterations needed to reach convergence. 
Thus, $DI_A = O(|X|^2\Delta_X (|C| + \tau))$.

\subsection{Adjusting the I-Index ($II$)}

I-Index \cite{maulik02tpami} is defined as 
\[
II(C, X, d) = \left(\frac{1}{|C|} \cdot \frac{\displaystyle \sum_{x\in X}d(x, c)}{\displaystyle \sum_{i=1}^{|C|}\sum_{x\in C_i}d(x, c_i) } \cdot \max_{1 \leq i, j \leq |C|} d(c_i, c_j)\right) ^ p,
\]
where $p$ is a constant that controls the discrimination between good and bad-quality clusterings, where we set $p=1$ for the rest of the adjustment.  
$II$ satisfies data-cardinality invariance but does not satisfy remaining invariance axioms. The adjustment procedure is as follows:

\noindent
\textbf{Applying T2 (Shift invariance)} 
As both the denominator and the numerator of the main fractional term are type-2 distances, we can easily make the term shift-invariant by (1) changing the distance function to the square of the Euclidean distance (T2-c), then by (2) converting the sum of distances into the average (T2-b), then applying the exponential function normalized by $\sigma_{d^2}$ (T2-a). 
On the other hand, we do not need an exponential protocol for the third term (max) as the term only consists of type-3 distances; we only divide it by $\sigma_{d^2}$ to ensure scale invariance. The resulting formula is as follows:
\begin{align*}
    II_1(C, X, d^2) =\frac{\displaystyle e^{\left(\displaystyle \sum_{x\in X}\frac{d^2(x, c)}{|X|\sigma_{d^2}} \right)}}{|C|\displaystyle e^{\left(\displaystyle \sum_{i=1}^{|C|}\sum_{x\in C_i}\frac{d^2(x, c_i) }{|X| \sigma_{d^2}}\right)}} \max_{1 \leq i, j \leq |C|} \frac{ d^2(c_i, c_j)}{\sigma_{d^2}}.
\end{align*}

\noindent
\textbf{Applying T4 (Range invariance)}
As $\max(II_1) \rightarrow + \infty$, we define $II_2 = 1/(1 + e^{-k \cdot II_1})$ so that $II_{2\max} \rightarrow 1$ (T4-b). As for $CH$ and $DI$, we get $II_3 = (II_2 - II_{2\min}) / (II_{2\max} - II_{2\min})$, where $II_{2\min} = E_{\pi}(II_2(C^{\pi}, X, d^2))$ (T4-a). The $k$ value are set by calibrating $II_3$ using human-judgment separability scores (T4-c).

\noindent
\textbf{Applying T3 (Class-cardinality invariance)} We design $II_A$ to be class-cardinality invariant by averaging class-pairwise scores:
\[
II_A = \frac{1}{{|C| \choose 2}} \sum_{S \subseteq C, |S|=2} II_3(C, X, d).
\]

\noindent
\textbf{Removing Monte-Carlo simulations} As we did for $CH_A$, we can accelerate the computation of $II_A$ by removing Monte-Carlo simulations for estimating $II_{2\min}$. As randomly permuting class labels makes every $C_i \in C$ satisfy $C_i \overset{D}{=} X$, $c \simeq c_i \forall c_i$. Therefore $d^2(c_i, c_j) \simeq 0$, which leads to $II_{1}(C^\pi, X, d^2) \simeq 0$ and $II_{2\min}= E_{\pi}(II_2(C^{\pi}, X, d)) = E_{\pi} (1/2) = 1/2$.

\noindent
\textbf{Computational Complexity}
$II$, $II_1$, $II_2$ is $O(|X|\Delta_X)$, thus $II_{2\min} = O(|X|\Delta_X T)$, where $T$ is the number of Monte Carlo simulations to compute $II_{2\min}$. $II_3$ is thus $O(|X|\Delta_X T)$ and $II_A = O(|X|\Delta_X T |C|)$. Removing the Monte-Carlo simulations reduces the complexity of $II_A$ to $O(|X|\Delta_X |C|)$.

\subsection{Adjusting Xie-Beni index ($XB$)}

Xie-Beni Index \cite{xie91tpami} is defined as:
\[
 XB(C, X, d^2) = \frac{\sum_{i=1}^{|C|}\sum_{x \in C_i}  d^2(x, c_i)}{|X| \cdot \min_{1\leq i, j \leq |C|, i \neq j}d^2(c_i, c_j)}.
\]
$XB$ misses all axioms except data-cardinality invariance. For the adjustment, we first take the inverse formula so that the higher score implies better clustering, resulting in:
\[
XB_1(C, X, d^2) = \frac{|X| \cdot \min_{1\leq i, j \leq |C|, i \neq j}d^2(c_i, c_j)}{\sum_{i=1}^{|C|}\sum_{x \in C_i}  d^2(x, c_i)}
\]

\noindent
\textbf{Applying T2 (Shift invariance)} 
As the denominator consists of type-2 distance while the numerator consists of type-3 distance, we add a factor term with type-2 distances to the numerator to equalize shifting. As we did for $CH$, we add the sum of squared distances of the data points to their centroid. 
We also remove the $|X|$ term from the numerator to ensure the data-cardinality invariance.
This leads to the following:
\[
 XB_2(C, X, d^2) = \frac{\displaystyle \sum_{x \in X} d^2(x, c)}{\displaystyle \sum_{i=1}^{|C|}\sum_{x \in C_i}  d^2(x, c_i)}\cdot \min_{1\leq i, j \leq |C|, i \neq j}d^2(c_i, c_j).
\]
We then apply the exponential protocol (T2-a, b) to the first term, while maintaining the second term as type-3 distances do not shift (we only normalized it by $\sigma_{d^2}$ to ensure scale-invariance). 
{
\small
\begin{align*}
 XB_3(C, X, d^2) = \frac{\exp\left({\displaystyle\sum_{x \in X} \frac{d^2(x, c)}{|X|\sigma_{d^2}}}\right)}{\exp\left({\displaystyle \sum_{i=1}^{|C|}\sum_{x \in C_i} \frac{d^2(x, c_i)}{|X|\sigma_{d^2}}}\right)}\min_{\substack{1\leq i, j \leq |C|\\ i \neq j}}\frac{d^2(c_i, c_j)}{\sigma_{d^2}}.
\end{align*}
}

\sloppy
Here, when we limit $|C|=2$, $XB_3(C, X, d^2) = 2 \cdot II_1 (C, X, d^2)$, as
$\min_{1\leq i, j \leq 2, i \neq j}d^2(c_i, c_j) =\max_{1 \leq i, j \leq 2} d^2(c_i, c_j) = d^2(c_1, c_2) $. 
Therefore, by applying to $XB_3$ the adjustment procedure of $II_1$, we  obtain $XB_A$ which is identical to $II_A$:

$$ \forall C, X, \quad XB_A(C, X, d^2) = II_A(C, X, d^2)$$

\fussy

\subsection{Adjusting Davies-Bouldin Index ($DB$)}

Davies-Bouldin index \cite{davies79tpami} is defined as:
\[
DB(C, X, d) = \frac{1}{|C|} \sum_{i=1}^{|C|} \max_{\substack{1\leq j\leq|C|\\ i \neq j}} \frac{\displaystyle\sum_{k \in \{i, j\}}\frac{1}{|C_k|} \sum_{x \in C_k} d(x, c_k)}{d(c_i, c_j)}.
\]
$DB$ satisfies data-cardinality invariance but misses all other across-dataset axioms. We first inverse the formula, making higher scores imply better clustering (i.e., $DB_1(C, X, d) = DB(C, X, d)^{-1}$).

\noindent
\textbf{Applying T2 (Shift invariance)}
As the denominator use type-3 distances while the numerator consists of type-2 distances, we add an additional term consisting of type-2 distances to the denominator and change the distance function to $d^2$ to equalize shifting. We add the average of squared distances of data points to their centroid, resulting in:
{
\small
\begin{align*}
&DB_2(C, X, d^2) =\left(
\displaystyle\frac{1}{|C|} \sum_{i=1}^{|C|} \max_{\substack{1\leq j\leq|C|\\ i \neq j}} \frac{\displaystyle\sum_{k \in \{i, j\}}\frac{1}{|C_k|}\sum_{x \in C_k} d^2(x, c_k)}{\displaystyle \frac{d^2(c_i, c_j)}{|X|}\sum_{x \in X} d^2(x, c)  
}\right)^{-1} 
\end{align*}
}

We then apply the exponential protocol (T2-a, b) to the first fractional term, while only normalizing the second term with $\sigma_{d^2}$ to ensure  scale invariance:
{
\footnotesize
\begin{align*}
DB_3(C, X, d^2) = 
\left(
\frac{1}{|C|} \sum_{i=1}^{|C|} \max_{\substack{1\leq j\leq|C|\\ i \neq j}}\frac{\displaystyle \sum_{k \in \{i, j\}}e^{\displaystyle  \frac{1}{|C_k|}\sum_{x \in C_k} \frac{d^2(x, c_k)}{\sigma_{d^2}}}} {\displaystyle \frac{d^2(c_i, c_j)}{\sigma_{d^2}} e^{\displaystyle \frac{1}{|X|}\sum_{x \in X} \frac{d^2(x, c)}{  \sigma_{d^2}}}}  
\right)^{-1} 
\end{align*}
}

\noindent
\textbf{Applying T4 (Range invariance)}
We apply min-max scaling to make $DB_A$ range invariant. As $\max(DB_3) \rightarrow +\infty$, we transform the function by applying the logistic function (T4-b), resulting in $DB_4 = 1/(1+e^{-k\cdot DB_3})$, so that $DB_{4\max} \rightarrow 1$. We then get $DB_5 = (DB_4 - DB_{4\min}) / (DB_{4\max} - DB_{4\min})$, where $DB_{4\min} = E^\pi (DB_4(C^\pi, X, d^2)$. $k$ value is calibrated based on human-judgment separability scores (T4-c).

\noindent \sloppy
\textbf{Removing Monte-Carlo simulations}
We remove the Monte-Carlo simulation estimating $DB_{4\min}$ to further accelerate the computation. As randomly permuting class labels makes $C_i \overset{D}{=} X$ $\forall C_i \in C$, thus $c_i \simeq c_j$ and $d^2(c_i, c_j) \simeq 0$ $\forall c_i, c_j$, $DB_3(C^\pi, X, d^2) \simeq 0$, which leads to $DB_{4\min} = E^\pi (DB_4(C^\pi, X, d^2) = E^\pi(1/2) = 1/2$.

\fussy

\noindent
\textbf{Computational Complexity}
The computational complexity of $DB, DB_1, DB_2, DB_3$, and $DB_4$ is $O(|X|\Delta_X)$. Therefore $DB_{4\min} = O(|X|\Delta_X T)$ and $DB_A =  O(|X|\Delta_X T |C|)$ where $T$ is the number of Monte-Carlo simulations to compute $DB_{4\min}$. By removing the simulations, we can reduce the complexity of $DB_A$ to $O(|X|\Delta_X |C|)$.

\subsection{Adjusting the Silhouette Coefficient ($SC$)}

Silhouette Coefficient \cite{rousseeuw87jcam} is defined as:

\[
SC(C, X, d) = \frac{1}{|C|} \cdot \sum_{i=1}^{|C|} \frac{1}{|C_i|}\sum_{x \in C_i} \frac{b(x) - a(x)}{\max(b(x), a(x))}.
\]
For a data point $x \in C_I$, 
\[
a(x) = \frac{1}{|C_I| - 1}\sum_{y \in C_I, x \neq y} d(x, y),
\]
and 
\[
b(x) = \min_{1 \leq J \leq |C|, I \neq J}\frac{1}{|C_J|}\sum_{y \in C_J} d(x, y).
\]
As $SC$ satisfies data-cardinality invariance (A1) and range invariance (A4) (\autorefapp{app:proofs}), we only need to apply the shift (T2) and class-cardinality (T4) protocols.

\noindent
\textbf{Applying T2 (Shift invariance)} As $a(x)$ and $b(x)$ are already robust estimators of population statistics (T1) and also consist of type-1 distances, we simply apply the exponential protocol (T2-a,b) to the terms, resulting in:
\[
SC_1(C, X, d) =  \frac{1}{|C|} \cdot \sum_{i=1}^{|C|} \frac{1}{|C_i|}\sum_{x \in C_i} \frac{b'(x) - a'(x)}{\max(b'(x), a'(x))},
\]
where 
\[
 a'(x) = e^{a(x) / \sigma^{d}} \text{ and } b'(x) = e^{b(x) / \sigma^{d}}.
\]

\noindent
\textbf{Applying T3 (Class-cardinality invariance)} We make $SC_A$ satisfy class-cardinality invariance by averaging class-pairwise scores:
\[
SC_A(C, X, d) = \frac{1}{{|C| \choose 2}} \sum_{S \subseteq C, |S|=2} SC_1(C, X, d).
\]
While $SC$ misses two across-dataset axioms, $SC_A$ satisfies them all.

\noindent
\textbf{Computational Complexity} The complexity of $SC$ and $SC_1$ is $O(|X|^2\Delta_X)$, thus $SC_A = O(|X|^2\Delta_X |C|)$.
