# Supplementary material for: Measuring the Validity of Clustering Validation Datasets
Source: arXiv:2503.01097 source file (2025-03-03)
Supplement: Supplementary file 3 [file D_proof.tex]

\section{Theorems and Proofs}

\label{app:proofs}
% Remind where these theorems ares used in the main paper, which section?

\subsection{About the Shift of Distances}

Here, we prove the theorems about the shift of type-1 and type-2 distances, which form the bases of the equalizing shifting step of the shift protocol (\autoref{sec:tricks} T2-c).

\label{app:proofshift}

\begin{itemize}[leftmargin=0em]
    \setlength\itemsep{4pt}
    
    \item[] 
    \textbf{Theorem 1.} \textit{$\forall X' \subset X$,  $\forall \beta > 0$, and for any Euclidean distance functions $d_L$ and $d_H$ satisfying $d_H^2 = d_L^2 + \beta$, 
   we have $\sum_{x \in X'}d_H^2(x, c) = \sum_{x \in X'}d^2_L(x,c) + \beta/2$, where $c = \overline{X'}$.}
    \item[] 
    \textit{Proof.} According to Hopcroft \& Kannon \cite{hopcroft14foundations}, for any set of data points $X' \subset X$, the following equality holds:
    \[
        2n \cdot \sum_{x \in X'} d^2(x, c)  = \sum_{x \in X'}\sum_{y \in X'} d^2(x,y).
    \]
    Here,
    \begin{align*}
        2n \cdot \sum_{x \in X'} d_H^2(x, c) &= \sum_{x \in X'}\sum_{y \in X'} d^2_H(x,y). \\
                                            &= \sum_{x \in X'}\sum_{y \in X'} (d^2_L + \beta)(x,y) \\
                                            &= n^2\beta + \sum_{x \in X'}\sum_{y \in X'} d^2_L(x,y) \\
                                            &=  n^2\beta + 2n \cdot \sum_{x \in X'} d_L^2(x, c)  \\
                                            &= 2n \cdot \left(\frac{n\beta}{2} + \sum_{x \in X'} d_L^2(x, c) \right) \\
                                            &= 2n \cdot \sum_{x \in X'} \left(d_L^2(x, c) + \frac{\beta}{2}\right)
    \end{align*}
    Therefore, $\sum_{x \in X'}d_H^2(x, c) = \sum_{x \in X'}d^2_L(x,c) + \beta/2$. \hfill $\Box$

    \item[] \textbf{Theorem 2.} \textit{$\forall X', X'' \subset X$, $\forall \beta > 0$, and for any $d_L$ and $d_H$ satisfying $d_H^2 = d_L^2 + \beta$, we have $d^2_H(c', c'') = d^2_L(c', c'')$, where $c' = \overline{X'}$ and $c''= \overline{X''}$.}
    \item[]
    \textit{Proof.} According to Apostol \& Mnatsakanian \cite{apostol03amm}, the following equality holds for any set of points $X'$, $X''$:
    \begin{align*}
        d^2(c_1, c_2) =& \frac{1}{n_{X'}n_{X''}}\sum_{x \in X'}\sum_{y \in X''}d^2(x,y) \\ &- \frac{1}{2n_{X'}^2}\sum_{x \in X'}\sum_{y \in X'}d^2(x,y) \\ &-
        \frac{1}{2n_{X''}^2}\sum_{x \in X''}\sum_{y \in X''}d^2(x,y).
    \end{align*}
    Here, using Theorem 1,
    \begin{align*}
        d^2_H(c_1, c_2) =& \frac{1}{n_{X'}n_{X''}}\sum_{x \in {X'}}\sum_{y\in {X''}}d^2_H(x,y) \\ &- \frac{1}{2n_{X'}^2}\sum_{x \in X'}\sum_{y \in X'}d^2_H(x,y) \\ &-
        \frac{1}{2n_{X''}^2}\sum_{x \in {X''}}\sum_{y \in {X''}}d^2_H(x,y). \\ 
        =& \frac{1}{n_{X'}n_{X''}}\sum_{x \in {X'}}\sum_{y \in {X''}}(d^2_L + \beta)(x,y) \\&- \frac{1}{2n_{X'}^2}\sum_{x \in {X'}}\sum_{y \in {X'}}(d^2_L + \beta)(x,y) \\ &-
        \frac{1}{2n_{X''}^2}\sum_{x \in {X''}}\sum_{y \in {X''}}(d^2_L + \beta)(x,y). \\ 
        =& \frac{1}{n_{X'}n_{X''}}\sum_{x \in {X'}}\sum_{y\in {X''}}d^2_L(x,y) \\ &- \frac{1}{2n_{X'}^2}\sum_{x \in X'}\sum_{y \in X'}d^2_L(x,y) \\ &+ \beta - \beta/2 - \beta/2 -
        \frac{1}{2n_{X''}^2}\sum_{x \in {X''}}\sum_{y \in {X''}}d^2_L(x,y) \\
         =& \frac{1}{n_{X'}n_{X''}}\sum_{x \in {X'}}\sum_{y\in {X''}}d^2_L(x,y) \\ &- \frac{1}{2n_{X'}^2}\sum_{x \in X'}\sum_{y \in X'}d^2_L(x,y) \\ &-
        \frac{1}{2n_{X''}^2}\sum_{x \in {X''}}\sum_{y \in {X''}}d^2_L(x,y)  
        \\ =& d^2_L(c_1, c_2)
    \end{align*}
    
\end{itemize}

% \subsection{About 

\subsection{About Class-Cardinality Invariance}

% We achieve class-cardinality invariance by aggregating local measures class-pairwisely. Here, we prove that if the local measures satisfy the remaining axioms (Shift invariance, range invariance, and data-cardinality invariance), the aggregated global measure also satisfies the axioms.

\label{app:proofclasscard}

\sloppy
Ackerman and Ben-David \cite{bendavid08nips} showed that if a function $f'$ satisfies any of the within-dataset axioms, then its aggregation $f(C, X, \delta)  = \textrm{agg}_{S \subseteq C, |S| = 2} f'(S, X, \delta)$ with $\textrm{agg}\in\{\min,\textrm{avg},\max\}$, also satisfies that axiom, which is represented by the following theorem from \cite{bendavid08nips}: 

\fussy

\begin{itemize}[leftmargin=0em]
    \setlength\itemsep{4pt}
    \item[] \textbf{Theorem 3.} \textit{If $f'$ satisfies a within-dataset axiom, then $\forall \textrm{agg}\in\{\min,\textrm{avg},\max\}, f(C, X, \delta)  = \textrm{agg}_{S \subseteq C, |S| = 2} f'(S, X, \delta)$ also satisfies the axiom.} \cite{bendavid08nips}
\end{itemize}

Here, we use Theorem 3 to prove the same property for across-dataset axioms.

\begin{itemize}[leftmargin=0em]
    \setlength\itemsep{4pt}
    \item[] \textbf{Theorem 4.} \textit{If $f'$ satisfies data-cardinality invariance (A1), then $f(C, X, \delta)  = \textrm{agg}_{S \subseteq C, |S| = 2} f'(S, X, \delta)$ is also data-cardinality invariant.}
    \item[] \sloppy
    \textit{Proof.} At first, $f(C, X, \delta) = \textrm{agg}_{S \subseteq C, |S| = 2} f'(S, X, \delta) $ and $f(\underline{C}_\alpha, X_\alpha, \delta) = \textrm{agg}_{S \subseteq \underline{C}_\alpha, |S| = 2} f'(S, X_\alpha, \delta) $ by definition (A3). Then, as  $\textrm{agg}_{S \subseteq C, |S| = 2} f'(S, X, \delta) = \textrm{agg}_{S \subseteq \underline{C}_\alpha, |S| = 2} f'(S, X_\alpha, \delta)$ (A1), $f(C, X, \delta) = f'(\underline{C}_\alpha, X_\alpha, \delta)$.
    Thus, $f$ satisfies data-cardinality invariance. \hfill $\Box$

    \fussy
    \item[] \sloppy \textbf{Theorem 5.} \textit{If $f'$ satisfies shift invariance, then $f(C, X, \delta)  = \textrm{agg}_{S \subseteq C, |S| = 2} f'(S, X, \delta)$ is also shift-invariant (A2).}
    \item[] \textit{Proof.} By definition (A3), $f(C, X, \delta) = \textrm{agg}_{S \subseteq C, |S| = 2} f'(S, X, \delta)$ and $f(C, X, \delta + \beta) = \textrm{agg}_{S \subseteq C, |S| = 2} f'(S, X, \delta + \beta)$. Then, as $\textrm{agg}_{S \subseteq C, |S| = 2} f'(S, X, \delta) = \textrm{agg}_{S \subseteq C, |S| = 2} f'(S, X, \delta + \beta)$ (A1), $f(C, X, \delta) = f(C, X, \delta + \beta)$. 
    Thus, $f$ satisfies shift invariance.  \hfill $\Box$

    \fussy
    \item[] \textbf{Theorem 6.} \textit{If $f'$ is range invariant over any pair of classes, then $f(C, X, \delta)  = \textrm{agg}_{S \subseteq C, |S| = 2} f'(S, X, \delta)$ is also Range Invariant (A4).}
    \item[] \sloppy \textit{Proof.} Assume $f'$ satisfies Range Invariance; i.e.,

    \[
        \forall S \subseteq C, |S| = 2, f'_{\min}(S,X,\delta)=0 \text{ and } f'_{\max}(S,X,\delta)=1.
    \]
    \fussy
    
     % We want to show that $f_{\min}=\min_C$$(\textrm{agg}_{S \subseteq C, |S| = 2}$$(f'(S,X,\delta)))=0$ and $f_{\max}=\max_C(\textrm{agg}_{S \subseteq C, |S| = 2}(f'(S,X,\delta)))=1$, with $\textrm{agg}\in\{\min,\textrm{avg},\max\}$. \\ 
    From the assumption, we get the following:
    \begin{itemize}[leftmargin=1em]
        \item[](1) $\min_S(f'_{\min})\leq\min_S(f')\leq \min_S(f'_{\max})$ so $\min_S(f')\in[0,1]$
        \item[](2) $\max_S(f'_{\min})\leq\max_S(f')\leq \max_S(f'_{\max})$ so $\max_S(f')\in[0,1]$
        \item[](3)  $\textrm{avg}_S(f'_{\min})\leq\textrm{avg}_S(f')\leq \textrm{avg}_S(f'_{\max})$ so $\textrm{avg}_S(f')\in[0,1]$

    \end{itemize}
    \fussy
    From (1), (2), and (3), we get $\forall C, \forall\textrm{agg}\in\{\min,\textrm{avg},\max\},\\ \textrm{agg}_{S \subseteq C, |S| = 2}(f'(S,X,d))\in[0,1]$
and so $f_{\min}=0$ and $f_{\max}=1$. Thus, $f$ satisfies Range Invariance if $f'$ does so. \hfill $\Box$
    
\end{itemize}

%\textit{Proof.} %Consider $C' = \arg \min_C f'(C, X, d)$ (i.e., $f'(C', X, d) = 0$). Then, for each subset $S$ of $C'$ satisfying $|S|=2$, $f'(S, X, d) = 0$ as $C$ is the worst possible clustering and modifying $C'$ will cause the increment of the score. Therefore, $\min_C f(C, X, d) = f(C', X, d) = \textrm{agg}_{S \subseteq C', |S| = 2} f'(S, X, d) = 0$. 
%In the same way, $\max_C f(C, X, d) = 1$.
%Thus, $f$ is Range Invariance. \hfill $\Box$

\subsection{About Baseline IVMs and Across-Dataset Axioms}

Our main claim is that standard IVM cannot properly evaluate and compare CLM across datasets as they do not satisfy the across-dataset axioms. We provide the proofs verifies the claim.

\subsubsection{About Calinski-Harabasz Index ($CH$)}
\hfill\\

$CH$ \cite{calinski74cis} is defined as:
\[
 CH(C, X, d^2) = \displaystyle\frac{|X| - |C|}{|C| - 1}\cdot\frac{\sum_{i=1}^{|C|}|C_i|d^2(c_i, c)}{\sum_{i=1}^{|C|} \sum_{x \in C_i} d^2(x, c_i)}, 
\]

\begin{itemize}[leftmargin=0em]
    \setlength\itemsep{4pt}

    \item[]
    \textbf{Theorem 7. } \textit{$CH$ does not satisfy data-cardinality invariance (W1). }
    \item[]
    \textit{Proof. }
    In the definition of $CH$, terms $d^2(c_i, c) / (|C| - 1)$ and \\$\sum_{i=1}^{|C|} \sum_{x \in C_i} d^2(x, c_i) / (|X| - |C|)$ are robust estimators of population statistics (average of distances; $|C|$ is the number of classes), thus robust to changes in data cardinality. However, the $|C_i|$ term in the numerator (amount of data in each class) makes $CH$ proportional to the number of points, thus making the function dependent on the data cardinality. \hfill $\Box$
    \item[] 
    \textbf{Theorem 8. } \textit{$CH$ does not satisfy shift invariance (W2). }
    \item[] 
    \textit{Proof. } 
    For any clustering $C$ over $(X, d)$, 
    \begin{align*}
    CH(C, X, d^2 + \beta) &= \frac{|X| - |C|}{|C| - 1}\cdot\frac{|X|\beta+\sum\limits_{i=1}^{|C|}|C_i|d^2(c_i, c)  }{|X|\beta+\sum\limits_{i=1}^{|C|} \sum\limits_{x \in C_i} d^2(x, c_i)} \\ &\neq CH(C, X, d)
    \end{align*}

    $CH$ does not satisfy Shift Invariance.
    \hfill $\Box$
    \item[]
    \textbf{Theorem 9}. \textit{$CH$ does not satisfy class-cardinality invariance (W3).}
    \item[]
    \textit{Proof.} $CH$ does not aggregate scores over pairs of clusters. Its formula cannot be algebraically transformed to an aggregation ($\min,\max,\textrm{avg}$) of cluster-pairwise formula. Therefore, $CH$ does not satisfy class-cardinality invariance by design.   \hfill $\Box$
    \item[] 
    \textbf{Theorem 10.} \textit{$CH$ does not satisfy Range Invariance (W4).}
    \item[]
    \textit{Proof. } The range of $CH$ is $[0, +\infty[$. Therefore, $CH$ is not range invariant as its maximum value is not bounded. \hfill $\Box$
\end{itemize}

\subsubsection{About Dunn Index ($DI$)}

\hfill\\

Dunn Index is defined as 
    \[
    DI(C, X, d) = \frac{\displaystyle \min_{C_i \in C} \min_{C_j \in C, C_i \neq C_j} \min_{x \in C_i, y \in C_j} d(x,y)}{\displaystyle \max_{C_k \in C} \max_{x, y \in C_k, x \neq y} d(x,y)}.
    \]

\begin{itemize}[leftmargin=0em]
    \setlength\itemsep{4pt}

    \item[] 
    \textbf{Theorem 11.} \textit{$DI$ does not satisfy data-cardinality invariance (A1).}

    \item[] 
    \textit{Proof.} 
    $DI$ is a fraction of minimum inter-cluster distances and maximum intra-cluster distances. The minimum and maximum functions are not robust to subsampling, there value can change drastically if the current min or max is not part of the subsample. Thus, $DI$ is not data-cardinality invariant. \hfill $\Box$

    \item[]
    \textbf{Theorem 12. } \textit{$DI$ does not satisfy Shift Invariance (A2).}

    \item[]
    \textit{Proof. } 
    \begin{align*}
    DI(C, X, d + \beta) &= \frac{\beta+\min\limits_{C_i \in C} \min\limits_{\substack{C_j \in C\\ i \neq j}} \min\limits_{\substack{x \in C_i\\ y \in C_j}} d(x,y) }{\beta+\max\limits_{C_k \in C} \max\limits_{\substack{x, y \in C_k\\ x \neq y}} d(x,y)} \\ &\neq DI(C, X, d).
    \end{align*}
    \hfill $\Box$.

    \item[]
    \textbf{Theorem 13. } \textit{$DI$ does not satisfy class-cardinality invariance (A3).}
    
    \item[]
    \textit{Proof.} $DI$ does not aggregate scores over pairs of clusters. Its formula cannot be algebraically transformed to an aggregation ($\min,\max,\textrm{avg}$) of cluster-pairwise formula. Therefore, $DI$ does not satisfy class-cardinality invariance by design. \hfill $\Box$.

    \item[]
    \textbf{Theorem 14. } \textit{$DI$ does not satisfy Range Invariance (A4).} 

    \item[]
    \textit{Proof. } The range of $DI$ is $[0, +\infty[$. Therefore, $DI$ is not range invariant as its maximum value is not bounded. \hfill $\Box$.
    
\end{itemize}

\subsubsection{About I Index ($II$)}

I-Index is defined as 
\[
II(C, X, d) = \left(\frac{1}{|C|} \cdot \frac{\displaystyle \sum_{x\in X}d(x, c)}{\displaystyle \sum_{i=1}^{|C|}\sum_{x\in C_i}d(x, c_i) } \cdot \max_{1 \leq i, j \leq |C|} d(c_i, c_j)\right) ^ p,
\]
\begin{itemize}[leftmargin=0em]
    \setlength\itemsep{4pt}

    \item[]
    \textbf{Theorem 15} \textit{$II$ satisfies data-cardinality invariance (A1).}

    \item[]
    \textit{Proof.} For any $C$ over $(X,d)$,
    %\begin{align*}
    %   II(\underline{C}_\alpha, X_\alpha, d) &= \left(\frac{1}{|C|} \cdot \frac{\sum_{x\in X_\alpha}d(x, c)}{\sum_{i=1}^{|C|}\sum_{x\in \underline{C_i}_\alpha}d(x, c_i) } \cdot \max_{1 \leq i, j \leq |C|} d(c_i, c_j)\right) ^ p \\ 
    %   &=  \left(\frac{1}{|C|} \cdot \frac{\sum_{x\in X}d(x, c) \cdot \alpha}{\sum_{i=1}^{|C|}\sum_{x\in C_i}d(x, c_i) \cdot \alpha} \cdot \max_{1 \leq i, j \leq |C|} d(c_i, c_j)\right) ^ p \\
    %   &= II(C, X, d) 
    %\end{align*}
    II uses averages of distances towards the average (center of gravity) of each class ($c_i$) and of the whole set of points ($c$), and the maximum distance between such centers. Average is a robust estimator of population statistics. Thus, $II$ is data-cardinality invariant.
    \hfill $\Box$

    \item[]
    \textbf{Theorem 16. } 
     \textit{$II$ does not satisfy Shift Invariance (A2).}

    \item[]
    \textit{Proof. } For any $C$ over $(X,d)$,
    \begin{align*}
            II(C, X, d + \beta) &= \left(\frac{1}{|C|} \cdot \frac{|X|\beta+\sum_{x \in X} d(x, c) }{|X|\beta+\sum_{i = 1}^{|C_i|} \sum_{x \in C_i} d(x, c_i)} \right. \\ &\left.\cdot \left(\beta+\max_{_{1 \leq i, j \leq |C|}} d(c_i, c_j)\right)\right)^p 
            \neq II(C, X, d).\\
    \end{align*}
    \hfill $\Box$.

    \item[]
    \textbf{Theorem 17. } \textit{$II$ does not satisfy class-cardinality invariance (A3). }
    \item[]
    \textit{Proof.} $II$ does not aggregate scores over pairs of clusters. Its formula cannot be algebraically transformed to an aggregation ($\min,\max,\textrm{avg}$) of cluster-pairwise formula. Therefore, $II$ does not satisfy class-cardinality invariance by design \hfill $\Box$.
    \item[]
    \textbf{Theorem 18. } \textit{$II$ does not satisfy Range Invariance (A4).} 
    \item[]
    \textit{Proof. } The range of $II$ is $[0, +\infty[$. Therefore, $II$ is not range invariant as its maximum value is not bounded. \hfill $\Box$.
\end{itemize}

\subsubsection{About Xie-Beni Index ($XB$)}
\hfill\\

Xie-Beni Index is defined as:
\[
 XB(C, X, d^2) = \frac{\sum_{i=1}^{|C|}\sum_{x \in C_i}  d^2(x, c_i)}{|X| \min_{1\leq i, j \leq |C|, i \neq j}d^2(c_i, c_j)}.
\]

\begin{itemize}[leftmargin=0em]
    \setlength\itemsep{4pt}

    \item[]
    \textbf{Theorem 19.} \textit{$XB$ satisfies data-cardinality invariance (A1).}

    \item[]
    \textit{Proof.} 
   % For any $C$ over $(X, d)$,
   % \begin{align*}
  %     XB(\underline{C}_\alpha, X_\alpha, d) &= \frac{\sum_{i=1}^{|C|}\sum_{x \in \underline{C_i}_\alpha}  d^2(x, c_i)}{|X_\alpha| \cdot \min_{1\leq i, j \leq |C|, i \neq j}d^2(c_i, c_j) } \\ &= \frac{\sum_{i=1}^{|C|}\sum_{x \in C_i}  d^2(x, c_i) \cdot \alpha}{|X| \cdot \min_{1\leq i, j \leq |C|, i \neq j}d^2(c_i, c_j) \cdot \alpha} \\ &= XB(C, X, d).
  %  \end{align*}
     $XB$ uses averages of distances towards the average (center of gravity) of each class ($c_i$) and the minimum distance between such centers. Averages are robust estimators of population statistics. Thus, $XB$ is data-cardinality invariant. \hfill $\Box$

    \item[]
    \textbf{Theorem 20.} \textit{$XB$ does not satisfy shift invariance (A2).}

    \item[]
    \textit{Proof.}
    For any $C$ over $(X, d)$,
    \begin{align*}
        XB(C, X, d^2 + \beta) &= \frac{|X|\beta+\sum_{i=1}^{|C|}\sum_{x \in C_i} d^2(x, c_i) }{|X| \left(\beta+ \min\limits_{1\leq i, j \leq |C|, i \neq j} d^2(c_i, c_j)\right) } \\ &\neq XB(C, X, d^2).
    \end{align*}
    Thus, $XB$ does not satisfy Shift Invariance. \hfill $\Box$

    \item[]
    \textbf{Theorem 21.} \textit{$XB$ does not satisfy class-cardinality invariance (A3).}

    \item[]
    \textit{Proof. } $XB$ does not aggregate scores over pairs of clusters. Its formula cannot be algebraically transformed to an aggregation ($\min,\max,\textrm{avg}$) of cluster-pairwise formula. Therefore, $XB$ does not satisfy class-cardinality invariance by design. \hfill $\Box$.

    \item[]
    \textbf{Theorem 22. }\textit{$XB$ does not satisfy Range Invariance (A4). }

    \item[]
    \textit{Proof.}  The range of $XB$ is $[0, +\infty[$. Therefore, $XB$ is not range invariant as its maximum value is not bounded. \hfill $\Box$.
\end{itemize}

\subsubsection{About Davies-Bouldin Index ($DB$)}

\hfill\\
Davies-Bouldin index is defined as:
\[
DB(C, X, d) = \frac{1}{|C|} \displaystyle\sum_{i=1}^{|C|} \max_{1 \leq j \leq |C|, i \neq j} \frac{\displaystyle \sum_{k \in \{i, j\}}\frac{1}{|C_k|} \sum_{x \in C_k} d(x, c_k)}{d(c_i, c_j)}.
\]

\begin{itemize}[leftmargin=0em]
    \setlength\itemsep{4pt}

    \item[]
    \textbf{Theorem 23.} \textit{$DB$ satisfies data-cardinality invariance (A1).}

    \item[]
    \textit{Proof.}
    %For any $C$ over $(X, d)$,
    %\begin{align*}
    %    DB(\underline{C}_\alpha, X_\alpha, d) &= \frac{1}{|C|} \sum_{i=1}^{|C|} \max_{1 \leq j \leq |C|, i \neq j} \frac{\sum_{k \in \{i, j\}}\frac{1}{|\underline{C_k}_\alpha|} \sum_{x \in \underline{C_k}_\alpha} d(x, c_k)}{d(c_i, c_j)} \\ &= \frac{1}{|C|} \sum_{i=1}^{|C|} \max_{1 \leq j \leq |C|, i \neq j} \frac{\sum\limits_{k \in \{i, j\}}\frac{1}{|C_k| \cdot \alpha} \sum_{x \in C_k} d(x, c_k) \cdot \alpha}{d(c_i, c_j)}    
    %    \\ &= DB(C, X, d).
    %\end{align*}
     $DB$ uses averages of distances towards the average (center of gravity) of each class ($c_i$) and the minimum distance between such centers. Averages are robust estimators of population statistics. Thus, $DB$ satisfies data-cardinality invariance. \hfill $\Box$

    \item[]
    \textbf{Theorem 24.} \textit{$DB$ does not satisfy shift invariance (A2).}
    For any $C$ over $(X,d)$,
    {
    \small
    \begin{align*}
        &DB(C, X, d + \beta)\\  &= \frac{1}{|C|} \sum_{i=1}^{|C|} \max_{\substack{j \in \{1,\cdots,|C|\}\\ i \neq j}} \frac{\frac{1}{|C_i|} \sum\limits_{x \in C_i} d(x, c_i) + \frac{1}{|C_j|} \sum\limits_{x \in C_j} d(x, c_j) + 2\beta}{d(c_i, c_j) + \beta} \\ 
  &\neq DB(C, X, d).
    \end{align*}
    }
    Thus, $DB$ does not satisfy shift invariance.

    \item[]
    \textbf{Theorem 25.} \textit{$DB$ does not satisfy class-cardinality invariance (A3).}

    \item[]
    \textit{Proof.} $DB$ does not aggregate scores over pairs of clusters. Its formula cannot be algebraically transformed to an aggregation ($\min,\max,\textrm{avg}$) of cluster-pairwise formula. Therefore, $DB$ does not satisfy class-cardinality invariance by design. \hfill $\Box$

    \item[]
    \textbf{Theorem 26. }\textit{$DB$ does not satisfy Range Invariance (A4). }

    \item[]
    \textit{Proof. }  The range of $DB$ is $[0, +\infty[$. Therefore, $DB$ is not range invariant as its maximum value is not bounded. \hfill $\Box$.
\end{itemize}

\subsubsection{About Silhouette Coefficient ($SC$)}

\hfill\\
Silhouette Coefficient is defined as:

\[
SC(C, X, d) = \frac{1}{|C|} \cdot \sum_{i=1}^{|C|} \frac{1}{|C_i|}\sum_{x \in C_i} \frac{b(x) - a(x)}{\max(b(x), a(x))}.
\]
For a data point $x \in C_I$, 
\[
a(x) = \frac{1}{|C_I| - 1}\sum_{y \in C_I, x \neq y} d(x, y),
\]
and 
\[
b(x) = \min_{1 \leq J \leq |C|, I \neq J}\frac{1}{|C_J|}\sum_{y \in C_J} d(x, y).
\]
\begin{itemize}[leftmargin=0em]
    \setlength\itemsep{4pt}

    \item[]
    \textbf{Theorem 27.} \textit{$SC$ satisfies data-cardinality invariance (A1).}

    \item[]
    \textit{Proof.} $a(x)$ and $b(x)$, two building blocks of $SC$, are both robust estimators of population statistics (average distances), and thus are data-cardinality invariance. Therefore, $SC$ is data-cardinality invariance.

    \item[]
    \textbf{Theorem 28.} \textit{$SC$ does not satisfy shift invariance (A2).}

    \item[]
    \textit{Proof.} For any $C$ over $(X, d)$,
    \begin{align*}
        SC(C, X, d + \beta) &= \frac{1}{|C|} \cdot \sum_{i=1}^{|C|} \frac{1}{|C_i|}\sum_{x \in C_i} \frac{b(x) - a(x)}{\beta + \max(b(x), a(x))} \\ &\neq SC(C,X, d).
    \end{align*}

    Thus, $SC$ is not shift invariant. \hfill $\Box$

    \item[]
    \textbf{Theorem 29.} \textit{$SC$ does not satisfy class-cardinality Invariance (A3).}

    \item[]
    \textit{Proof.} $SC$ does not aggregate scores over pairs of clusters. Its formula cannot be algebraically transformed to an aggregation ($\min,\max,\textrm{avg}$) of cluster-pairwise formula. Therefore, $SC$ does not satisfy class-cardinality invariance by design. \hfill $\Box$

    \item[]
    \textbf{Theorem 30. }\textit{$SC$ satisfies Range Invariance (A4). }

    \item[]
    \textit{Proof.} The theoretical range of $SC$ is $[-1, 1]$, and the expected minimum of the measure (based on randomly permuted class labels) is 0. Therefore, $SC$ is range invariant.

\end{itemize}

\subsection{About $CH_A$ and Across-Dataset Axioms}

\begin{itemize}[leftmargin=0em]
    \setlength\itemsep{4pt}

        \item[]
    \textbf{Theorem 31.} $CH_5$ satisfies data-cardinality invariance (A1).

    \item[]
    \textit{Proof.}
    $CH_A$ uses averages of distances towards the center of gravity of each class ($c_i$) or the entire dataset ($c$), or the average of distances between the centers. Averages are robust estimators of population statistics. Thus, $CH_5$ satisfies data-cardinality invariance. Due to Theorem 4, $CH_A$ is also data-cardinality invariant as it is the class-pairwise aggregation of $CH_5$.
    
    \hfill $\Box$

    \item[]
    \textbf{Theorem 32.} $CH_A$ satisfies shift invariance (A2).

    \item[]
    \textit{Proof.} For any $C$ over $(X, d)$,
    {
    \small
    \begin{align*}
        CH_{3}(C, X, d^2 + \beta) &= \displaystyle\frac{e^{\frac{\sum\limits_{x \in X} (d^2(x, c) + \beta)}{\sigma_{d^2} \cdot |X|}}}{e^{\frac{\sum\limits_{i=1}^{|C|} \sum\limits_{x \in C_i} (d^2(x, c_i)+\beta)}{ \sigma_{d^2} \cdot|X|}}} \cdot \frac{\sum\limits_{i=1}^{|C|}|C_i|(d^2(c_i, c) + \beta)}{\sigma_{d^2} \cdot|X| \cdot (|C| - 1)} \\
        &= \displaystyle\frac{e^{\frac{\sum\limits_{x \in X} d^2(x, c)}{\sigma_{d^2} \cdot |X|}} e^{\frac{\beta}{\sigma_{d^2}}}}{e^{\frac{\sum\limits_{i=1}^{|C|} \sum\limits_{x \in C_i} d^2(x, c_i)}{ \sigma_{d^2} \cdot|X|}}e^{\frac{\beta}{\sigma_{d^2}}}} \cdot \frac{\sum\limits_{i=1}^{|C|}|C_i|d^2(c_i, c)}{\sigma_{d^2} \cdot|X| \cdot (|C| - 1)} \\
        &= CH_3(C,X, d^2).
    \end{align*}
    }
    Therefore, $CH_3$ is shift invariant, thus $CH_4$ and $CH_5$ are also shift invariant. Due to Theorem 5, $CH_A$ is also shift invariant as it is the class-pairwise aggregation of $CH_5$. 
    \hfill $\Box$

    \item[]
    \textbf{Theorem 33.} $CH_A$ satisfies class-cardinality invariance (A3).

    \item[]
    \textit{Proof.} $CH_A$ is defined as the class-pairwise aggregation of $CH_5$, thus is class-cardinality invariant \hfill $\Box$.

    \item[]
    \textbf{Theorem 34.} $CH_A$ satisfies range invariance (A4)

    \item[]
    \textit{Proof.} The range of $CH_5$ is $[0,1]$. thus $CH_5$ is range invariant. Therefore, due to Theorem 6, $CH_A$ is also range invariant as it is the class-pairwise aggregation of $CH_5$. \hfill $\Box$

\end{itemize}
