# Supplementary material for: Measuring the Validity of Clustering Validation Datasets
Source: arXiv:2503.01097 source file (2025-03-03)
Supplement: Supplementary file 4 [file F_setting.tex]

\section{Experimental Setting}

\label{app:setting}

\noindent
\textbf{Classifiers settings } As aforementioned in Section 5.2., we exploited Bayesian Optimization \cite{snoek12neurips} to find the best hyperparameter setting of the classifiers for each fold of cross validation. We used the implementation of Nogueira \cite{nogueira14github}. For each classifiers, we performed five random exploration and 25 steps of optimization, following the default setting of the implementation. For the bounds of the hyperparameters, we exploited the settings provided by \texttt{auto-sklearn} \cite{feurer15nips}. For the hyperparameters that are not mentioned below, we used the default provided by \texttt{sklearn}. 
\begin{itemize}
    \item \textbf{Support Vector Machine} (SVM)
    \begin{itemize}
        \item \texttt{C}: [$2^{-5}, 2^{5}$]
        \item \texttt{gamma}: [$2^{-15}, 2^3$]
    \end{itemize}
    \item \textbf{$k$-Nearest Neighbor} ($k$NN)
    \begin{itemize}
        \item \texttt{n\_neighbors}: [1, $2 \cdot \sqrt{\text{|X|}}$], where $|X|$ denotes the number of data points
    \end{itemize}
    \item \textbf{Multilayer Perceptron} (MLP)
    \begin{itemize}
        \item \texttt{hidden\_layer\_depth}: [1, 4]
        \item \texttt{num\_nodes\_per\_layer}: [16, 256]
        \item \texttt{activation}: \{\texttt{identity}, \texttt{logistic}, \texttt{tanh}, \texttt{relu}\}
        \item \texttt{alpha}: [$10^{-7}, 10^{-1}$]
        \item \texttt{learning\_rate\_init}: [$10^{-4}$, 0.5]
    \end{itemize}
    \item \textbf{Naive Bayesian networks} (NB)
    \begin{itemize}
        \item \texttt{var\_smoothing}: [$10^{-12}, 1$]
    \end{itemize}
    \item \textbf{Random forest} (RF)
    \begin{itemize}
        \item \texttt{n\_estimators}: [1, 200]
        \item \texttt{min\_samples\_split}: [2, 20]
        \item \texttt{min\_samples\_leaf}: [1, 20],
        \item \texttt{criterion}: \{\texttt{gini}, \texttt{entropy}, \texttt{log\_loss}\}
    \end{itemize}
    \item \textbf{Logistic regression} (LR)
    \begin{itemize}
        \item \texttt{penalty}: \{\texttt{L1}, \texttt{L2}, \texttt{Elasticnet}\}
        \item \texttt{C}: [$2^{-5}, 2^{5}$]
        \item \texttt{tol}: [$10^{-5}, 10^{-1}$]
        \item \texttt{l1\_ratio}: [0, 1]
    \end{itemize}
    \item \textbf{Linear discriminant analysis} (LDA)
    \begin{itemize}
        \item \texttt{tol}: [$10^{-5}, 10^{-1}$]
        \item \texttt{solver}: \{\texttt{svd}\}
    \end{itemize}
\end{itemize}

For the ensemble of classifiers, we used the max combination of the classifiers (i.e., chose the highest score among the classifiers). Finally, we estimated the CLM ranking of the labeled datasets based on the classification scores.

\noindent
\textbf{Settings for computing ground-truth CLM.}
We used \texttt{sklearn} implementation for DBSCAN, $K$-Means, Birch, Agglomerative clustering, and used \texttt{sklearn-extra} implementation for $K$-Medoids. We used \texttt{pyclustering} implementation for $X$-Means. For HDBSCAN, we used the implementation of McInnes et al. \cite{mcinnes17oss}. 
To find the best hyperparameter setting for each clustering technique, we used Nogueira's Bayesian optimization implementation \cite{nogueira14github} with default setting, as we did for classification techniques. 
The bounds of each technique's hyperparameter is set as follows:
\begin{itemize}
    \item \textbf{DBSCAN}
    \begin{itemize}
        \item \texttt{epsilon}: [0.01, 1.0]
        \item \texttt{min\_samples}: [1, 10]
    \end{itemize}
    \item \textbf{HDBSCAN}
    \begin{itemize}
        \item \texttt{epsilon}: [0.01, 1.0]
        \item \texttt{min\_samples}: [1, 10]
        \item \texttt{min\_cluster\_size}: [2, 50]
    \end{itemize}
    \item \textbf{\textit{K}-Means}
    \begin{itemize}
        \item $K$ (number of clusters): [2, $|C| \cdot$ 3], where $|C|$ denotes the number of classes in data
    \end{itemize}
    \item \textbf{\textit{K}-Medoids}
    \begin{itemize}
        \item $K$: [2,  $ |C| \cdot$ 3]
    \end{itemize}
    \item \textbf{\textit{X}-Means}
    \begin{itemize}
        \item \texttt{kmax}: [2, 50]
        \item \texttt{tolerance}: [0.01, 1.0]
    \end{itemize}
    \item \textbf{Birch}
    \begin{itemize}
        \item \texttt{threshold}: [0.1, 1.0]
        \item \texttt{branching\_factor}: [10, 100]
    \end{itemize}
    \item \textbf{Agglomerative Clustering}
    \begin{itemize}
        \item number of clusters: [2, $ |C| \cdot$ 3]
    \end{itemize}
\end{itemize}

We used Single, Average, and Complete variants of Agglomerative Clustering. After finding the best hyperparameter setting of a clustering technique for a given datasets, we ran the technique 20 times with the same setting and report the average value as the final score.
