# Supplementary material for: Measuring the Validity of Clustering Validation Datasets
Source: arXiv:2503.01097 source file (2025-03-03)
Supplement: Supplementary file 6 [file B_calibration.tex]

\section{Alleviating the Imbalance of Human-driven Separability Scores}

\label{app:calibration}

We use the human-driven separability score of Gaussian clusters \cite{abbas19cgf, AupetitVIS19} to calibrate the logistic growth rate $k$ of \IVMa (\autoref{sec:trick4} T4-c) and compute the error in the ablation study (\autoref{sec:validity}). We need to weigh each separability score to compensate for their non-uniform distribution. Here we provide a pseudo-code for computing these weights. Note that we assume that the scores range between 0 and 1 (\autoref{algo:weight}).

\RestyleAlgo{ruled}
\SetKwComment{Comment}{/* }{ */}

\begin{algorithm}

\caption{Assigning weights to each dataset to compensate for the imbalance of human-driven separability scores}\label{algo:weight}
\KwIn{list of scores $S = [s_1, s_2, \cdots, s_n]$ with length $n$}
\KwIn{number of bins $b$}
\KwOut{list of weights $W = [w_1, w_2, \cdots, w_n]$}
$bins = []$, $w\_bins = []$ \Comment*[r]{initialize empty list}
\For{$i=1$ \KwTo $b$}{
    $bins$.\textbf{append}(0) \Comment*[r]{create bins}
}
$bin\_size = 1 / b$ \;
\For{$k=1$ \KwTo $n$}{ 
    $bin\_idx = \lceil s_k / bin\_size \rceil$\Comment*[r]{quantize scores} 
    $bins[bin\_idx] += 1$\Comment*[r]{count frequencies} 
}
\For{$i=1$ \KwTo $b$}{
$w\_bins[i] = 1 / bins[i]$  \Comment*[r]{compute bin weights}
}
$W = []$ \;
\For{$k=1$ \KwTo $n$}{
    $W.$\textbf{append}$(w\_bins[\lceil s_k / bin\_size \rceil])$
}
\KwRet{$W$}
\end{algorithm}
