# Supplementary material for: Measuring the Validity of Clustering Validation Datasets
Source: arXiv:2503.01097 source file (2025-03-03)
Supplement: Supplementary file 7 [file E_gaussian_datasets.tex]

\section{Base Gaussian Datasets}

For the ablation study (\autoref{sec:validity}) and logistic growth rate calibration (\autoref{sec:trick4} T4-c), we used datasets where each consisting of two Gaussian clusters with diverse hyperparameters. \autoref{fig:basis} shows a subset of 28 scatterplot representations of these datasets among 1000 available.

\begin{figure}[t]
    \centering
    \includegraphics[width=\linewidth]{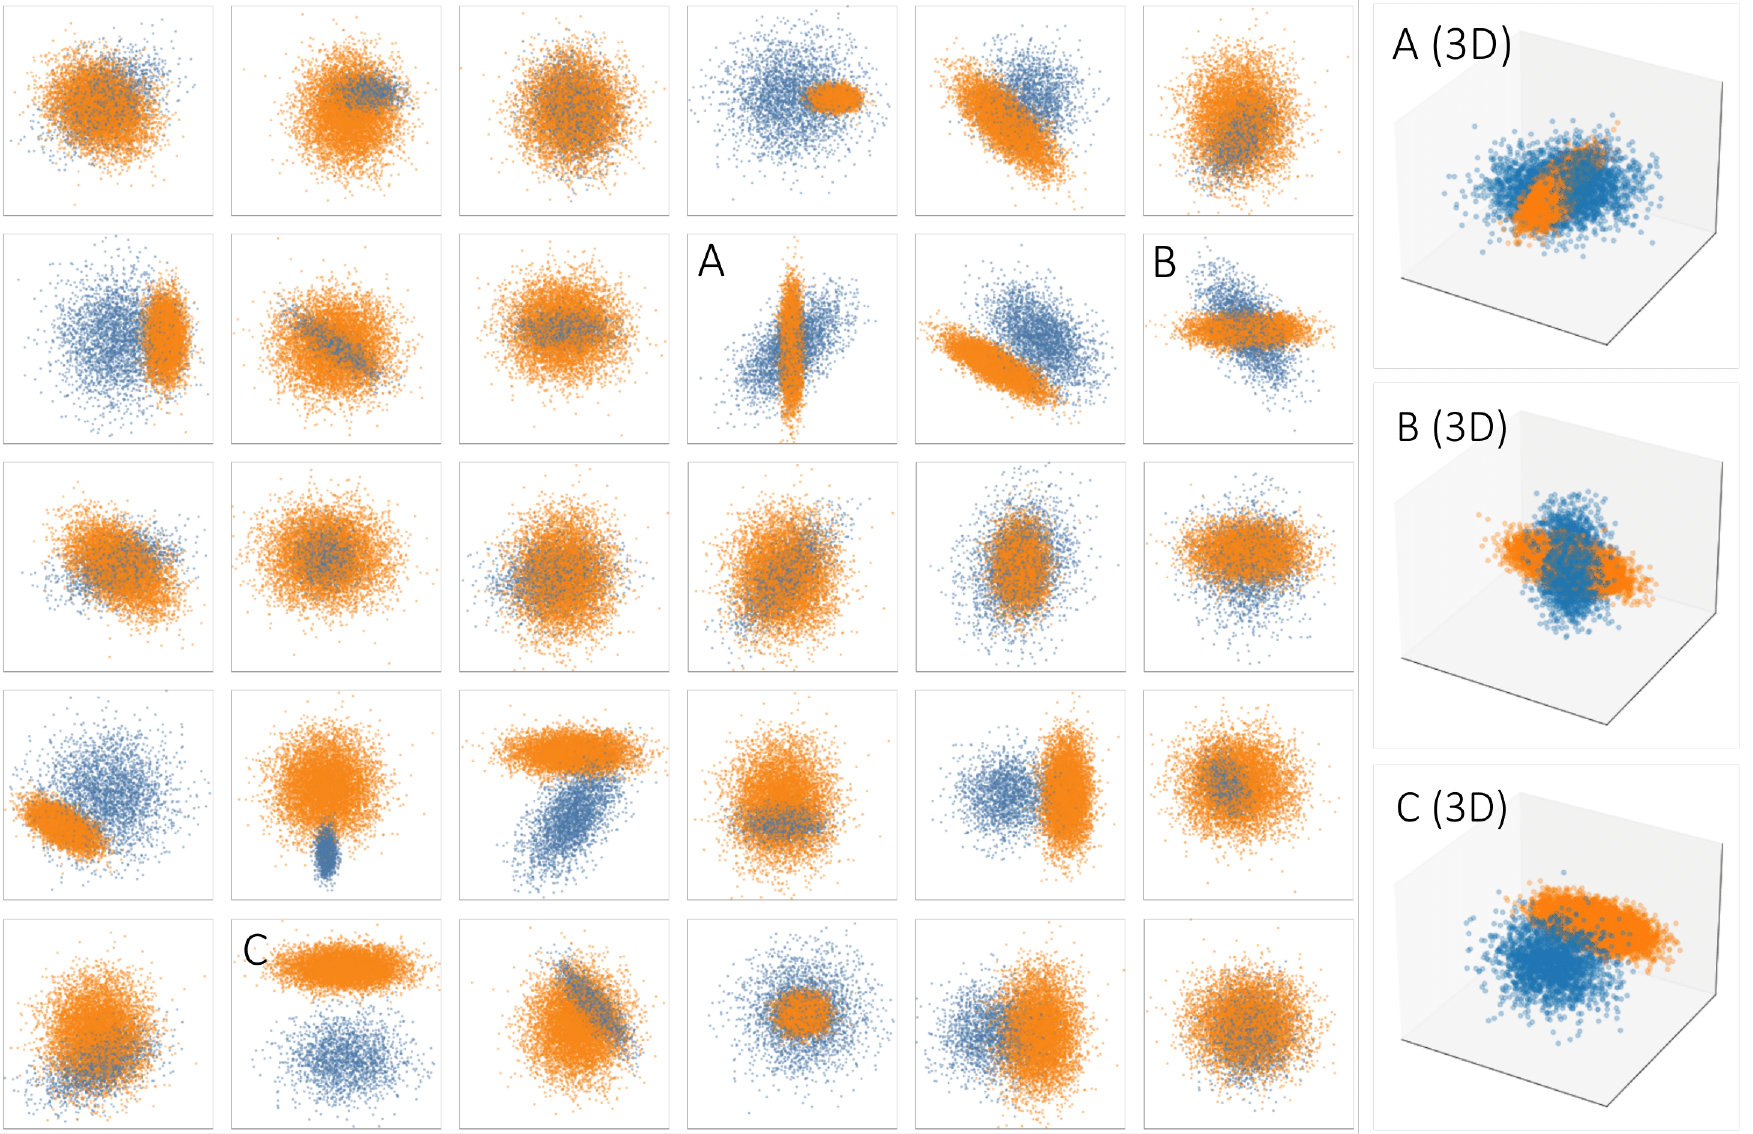}
    \vspace{-5mm}
    \caption{Subset of 1,000 base datasets used in the ablation study (\autoref{sec:validity})  and logistic growth rate calibration (\autoref{sec:trick4} T4-c); we displayed the first two (left) and three (right) axes of each dataset. Note that only the first two axes are used to calibrate the logistic growth rate of \IVMa.
    }
    \label{fig:basis}
\end{figure}
