# Supplementary material for: Measuring the Validity of Clustering Validation Datasets
Source: arXiv:2503.01097 source file (2025-03-03)
Supplement: Supplementary file 8 [file main_with_appendix.tex]

\documentclass[compsoc]{IEEEtran}
\usepackage{amsmath,amsfonts}
\usepackage{algorithmic}
\usepackage{array}
\usepackage[caption=false,font=normalsize,labelfont=sf,textfont=sf]{subfig}
\usepackage{textcomp}
\usepackage{stfloats}
\usepackage{url}
\usepackage{verbatim}
\usepackage{graphicx}
\usepackage{cite}
\hyphenation{op-tical net-works semi-conduc-tor IEEE-Xplore}
% updated with editorial comments 8/9/2021

\usepackage{multicol}
\usepackage{multirow}
\usepackage{xcolor,colortbl}
\usepackage{xspace}
\usepackage{enumitem}
\usepackage{makecell}
\usepackage{booktabs}
\usepackage{hyperref}
\usepackage{algorithm2e}
\usepackage{mathtools} 
\usepackage{amssymb}
\usepackage{amsmath}

\newcommand{\autorefapp}[1]{\hyperref[#1]{Appendix~\ref*{#1}}}

 % Jan Hlavacek

\definecolor{cbblue}{RGB}{0, 114, 178}
\definecolor{cbgreen}{RGB}{0, 158, 115}
\definecolor{cbred}{RGB}{213, 94, 0}
\definecolor{cbbrown}{RGB}{124, 65, 28}

\def\IVMa{IVM$_{A}$\xspace}
 % shortcut for Ackerman and Ben-David

\begin{document}

\title{Measuring the Validity of \\ Clustering Validation Datasets}

\author{Hyeon Jeon, Micha\"el Aupetit, DongHwa Shin, Aeri Cho, Seokhyeon Park, and Jinwook Seo
        % <-this % stops a space
\thanks{Hyeon Jeon, Aeri Cho, Seokhyeon Park, and Jinwook Seo are with Seoul National University. e-mail: \{hj, archo, shpark\}@hcil.snu.ac.kr, jseo@snu.ac.kr}% <-this % stops a space
\thanks{Micha\"el Aupetit is with Qatar Computing Research Institute, Hamad Bin
Khalifa University. e-mail: maupetit@hbku.edu.qa}
\thanks{DongHwa Shin is with Kwangwoon University. e-mail: dhshion@kw.ac.kr}
\thanks{Manuscript received April 19, 2021; revised August 16, 2021.}}

% The paper headers
\markboth{}%
{Jeon \MakeLowercase{\textit{et al.}}: Measuring the Validity of Clustering Validation Datasets}

\IEEEpubid{0000--0000/00\$00.00~\copyright~2021 IEEE}
% Remember, if you use this you must call \IEEEpubidadjcol in the second
% column for its text to clear the IEEEpubid mark.

\IEEEtitleabstractindextext{
\begin{abstract}
\input{sections/00_abstract}
\end{abstract}
\begin{IEEEkeywords}
Clustering, Clustering Validation, Internal Clustering Validation, External Clustering Validation, Clustering Benchmark
\end{IEEEkeywords}
}

\maketitle

\input{sections/01_introduction}
\input{sections/02_related_work}
\input{sections/03_axioms}
\input{sections/04_tricks}
\input{sections/05_generalization}
\input{sections/06_evaluation}
\input{sections/07_application}
\input{sections/08_discussion}
\input{sections/09_conclusion}

% \section*{Acknowledgments}
% This should be a simple paragraph before the References to thank those individuals and institutions who have supported your work on this article.

\bibliographystyle{IEEEtran}
\bibliography{ref}

% \appendices

% \newpage

\section{Ackerman \& Ben-David's \cite{bendavid08nips} Within-dataset Axioms }

\label{app:within}

\noindent
\textbf{(Axiom W1) \textit{Scale Invariance} } \textit{A measure $f$ satisfies scale invariance if for every clustering $C$ of $(X, d)$, and every positive $\alpha$, $f(C, X, d) = f(C, X, \alpha d)$ (where $\alpha d$ is defined by setting, for every pair of domain points $x, y$, $\alpha d(x,y) = \alpha \cdot d(x,y)$)
}

\noindent
\textbf{$C$-consistent variant (Used in W2)} \textit{Given a clustering $C$ over $(X, d)$, a distance function $d'$ is $C$-consistent variant of $d$, if $d'(x, y) \leq d(x,y)$ for all $x \sim_C y$, and $d'(x, y) \geq d(x,y)$ for all $ x \nsim_C y$.}

\noindent
\textbf{(Axiom W2) \textit{Consistency} } \textit{A measure $f$ satisfies consistency if for every clustering $C$ over $(X, d)$, whenever $d'$ is a $C$-consistent variant of $d$, then   $f(C, X, d') \geq f(C, X, d)$}

% The third axiom requires the measures to be rich; any clustering should have an opportunity to have a best score over the domain by modifying the distance function. 
\noindent
\textbf{(Axiom W3) \textit{Richness}} \textit{A measure $f$ satisfies richness if
for each non-trivial clustering $C$ of $X$, there exists a distance function $d$ over $X$ such that $X = \arg\max f(C_i, X, d)$.}

% The last axiom is added to prevent a function that consider the identity of domain points (e.g., relate class labels to the score) to be regarded as a within-dataset internal measure.
\noindent
\textbf{Clustering Isomorphism (Used in W4)} \textit{Two clustering $C$ and $C'$ over the same domain, $(X, d)$, are isomorphic, denoted $C \approx_d C' $, if there exists a distance-preserving isomorphism $\phi: X \rightarrow X$, such that for all $ x, y \in X$, $x \sim_C y$ if and only if $\phi(x) \sim_{C'} \phi(y)$.}

\noindent
\textbf{(Axiom W4) \textit{Isomorphism Invariance}} \textit{A measure $f$ is isomorphism invariant if for all clusterings $C, C'$ over $(X, d)$ where $C \approx_d C'$, $f(C, X, d) = f(C', X, d)$}

\section{Alleviating the Imbalance of Human-driven Separability Scores}

\label{app:calibration}

We use the human-driven separability score of Gaussian clusters \cite{abbas19cgf, AupetitVIS19} to calibrate the logistic growth rate $k$ of \IVMa (\autoref{sec:trick4} T4-c) and compute the error in the ablation study (\autoref{sec:validity}). We need to weigh each separability score to compensate for their non-uniform distribution. Here we provide a pseudo-code for computing these weights. Note that we assume that the scores range between 0 and 1 (\autoref{algo:weight}).

\RestyleAlgo{ruled}
\SetKwComment{Comment}{/* }{ */}

\begin{algorithm}

\caption{Assigning weights to each dataset to compensate for the imbalance of human-driven separability scores}\label{algo:weight}
\KwIn{list of scores $S = [s_1, s_2, \cdots, s_n]$ with length $n$}
\KwIn{number of bins $b$}
\KwOut{list of weights $W = [w_1, w_2, \cdots, w_n]$}
$bins = []$, $w\_bins = []$ \Comment*[r]{initialize empty list}
\For{$i=1$ \KwTo $b$}{
    $bins$.\textbf{append}(0) \Comment*[r]{create bins}
}
$bin\_size = 1 / b$ \;
\For{$k=1$ \KwTo $n$}{ 
    $bin\_idx = \lceil s_k / bin\_size \rceil$\Comment*[r]{quantize scores} 
    $bins[bin\_idx] += 1$\Comment*[r]{count frequencies} 
}
\For{$i=1$ \KwTo $b$}{
$w\_bins[i] = 1 / bins[i]$  \Comment*[r]{compute bin weights}
}
$W = []$ \;
\For{$k=1$ \KwTo $n$}{
    $W.$\textbf{append}$(w\_bins[\lceil s_k / bin\_size \rceil])$
}
\KwRet{$W$}
\end{algorithm}

\section{Generalization of Remaining IVMs}

\label{app:gener}

Here, we describe the adjustment process of the remaining IVMs, which we explain briefly in \autoref{sec:remaining}.

\subsection{Adjusting the Dunn Index ($DI$)}

Dunn Index \cite{dunn74joc} is defined as:
\[
DI(C, X, d) = \frac{\displaystyle \min_{1 \leq i \leq |C|} \min_{1 \leq j \leq |C|} \min_{x \in C_i, y \in C_j} d(x,y)}{\displaystyle \max_{1 \leq k \leq |C|} \max_{x, y \in C_k} d(x,y)}.
\]
$DI$ satisfies none of the across-dataset axioms; thus we applied every possible protocols we provided (\autoref{sec:tricks}). 

\noindent
\textbf{Applying T1 (Data-cardinality invariance)} Both the denominator (maximum intra-class distance) and numerator (minimum inter-class distance) of $DI$ compute the minimum or maximum over point pairwise distances, which is very sensitive to noise. We thus first change the denominator and numerator into the maximum average intra-class distance and minimum average inter-class distance, respectively, leading to:
\[
DI_1(C, X, d) = \frac{\displaystyle \min_{1 \leq i \leq |C|} \min_{1 \leq j \leq |C|} \frac{\sum_{x \in C_i, y \in C_j} d(x,y)}{|C_i| \cdot |C_j|}}{\displaystyle \max_{1 \leq k \leq |C|} \frac{\sum_{x, y \in C_k} d(x,y)}{(k \cdot (k - 1)) / 2}}.
\]

\noindent
\textbf{Applying T2 (Shift invariance)} As both denominator and numerator of $DI_1$ consist of type-1 distances, we can directly apply the exponential protocol, hence:
% \[
% DI_2(C, X, d) = \frac{(e^{\min_{1 \leq i \leq |C|} (\min_{1 \leq j \leq |C|} \frac{\sum_{x \in C_i, y \in C_j} d(x,y)}{|C_i| \cdot |C_j|})})^{1/\sigma_d}}{(e^{\max_{1 \leq k \leq |C|} \frac{\sum_{x, y \in C_k} d(x,y)}{(k \cdot (k - 1)) / 2}})^{(1 / \sigma_d)}},
% \]

\[
DI_2(C, X, d) = \frac{\displaystyle \exp\left(\frac{1}{\sigma_d}\min_{1 \leq i \leq |C|} \min_{1 \leq j \leq |C|} \frac{\displaystyle\sum_{x \in C_i, y \in C_j} d(x,y)}{|C_i| \cdot |C_j|}\right)}{\displaystyle \exp\left(\frac{1}{\sigma_d}\max_{1 \leq k \leq |C|} \frac{\displaystyle \sum_{x, y \in C_k} d(x,y)}{(k \cdot (k - 1)) / 2}\right)},
\]
where $\sigma_d = \text{std}(\{d(x,c)| x \in X\})$.

\noindent
\textbf{Applying T4 (Range invariance)}
In the case of maximum score, as $\max(DI_2) \rightarrow + \infty$, we apply the logistic function (T4-b), resulting in $DI_3 = 1/(1+ e^{-k \cdot DI_2})$, to achieve $DI_{3\max} \rightarrow 1$. As we did for $CH$, we estimate the worst score as the expectation of $DI_3$ over random clustering partitions $C^\pi$ (T4-a): $DI_{3\min} = E_\pi (DI_3(C^\pi, X, d))$. We then get $DI_4 = (DI_3 - DI_{3\min}) / (DI_{3\max} - DI_{3\min})$. We set the growth rate $k$ by calibrating $DI_4$ using human-judgement separability scores (T4-c).

\noindent
\textbf{Applying T3 (class-cardinality invariance)} As in $CH_A$ (\autoref{sec:gener}), we make $DI_A$ class-cardinality invariant by averaging class-pairwise scores:
\[
DI_A = \frac{1}{{|C| \choose 2}} \sum_{S \subseteq C, |S|=2} DI_4(C, X, d).
\]

\noindent\sloppy
\textbf{Approaching $DI_{3}$'s minimum bound}
We found that $DI_{3\min}$ can get closer to the minimum bound of $DI_{3}$ by defining $DI_{3\min} = DI_3(C^{\psi}, X, d)$; $C^{\psi} = \{C^{\psi}_1, C^{\psi}_2\}$ satisfying $|C^{\psi}_1| = \{x\}$ and $|C^{\psi}_2| = X \setminus \{x\}$ where $x$ is the geometric median of $X$ (i.e., $x = \arg\min_{x' \in  X} \sum_{y\in X} d(x',y)$). $DI_3(C^{\psi}, X, d)$  is always smaller than $DI_3(C^{\pi}, X, d)$, thus always closer to the worst case (Proof in \autorefapp{app:proofs}). 

\fussy

\noindent
\textbf{Computational Complexity}
The computational complexity of $DI$, $DI_1$, $DI_2$, $DI_3$ is $O(|X|^2\Delta_X)$. 
If we use the geometric median-based worst-case approximation, the performance of $DI_{3\min}$ also depends on the time complexity of the algorithm that computes the geometric median. We use the one proposed by Vardi and Zhang \cite{vardi00nas}; the complexity is $O(|X|\Delta_X \tau)$ where $\tau$ is the number of iterations needed to reach convergence. 
Thus, $DI_A = O(|X|^2\Delta_X (|C| + \tau))$.

\subsection{Adjusting the I-Index ($II$)}

I-Index \cite{maulik02tpami} is defined as 
\[
II(C, X, d) = \left(\frac{1}{|C|} \cdot \frac{\displaystyle \sum_{x\in X}d(x, c)}{\displaystyle \sum_{i=1}^{|C|}\sum_{x\in C_i}d(x, c_i) } \cdot \max_{1 \leq i, j \leq |C|} d(c_i, c_j)\right) ^ p,
\]
where $p$ is a constant that controls the discrimination between good and bad-quality clusterings, where we set $p=1$ for the rest of the adjustment.  
$II$ satisfies data-cardinality invariance but does not satisfy remaining invariance axioms. The adjustment procedure is as follows:

\noindent
\textbf{Applying T2 (Shift invariance)} 
As both the denominator and the numerator of the main fractional term are type-2 distances, we can easily make the term shift-invariant by (1) changing the distance function to the square of the Euclidean distance (T2-c), then by (2) converting the sum of distances into the average (T2-b), then applying the exponential function normalized by $\sigma_{d^2}$ (T2-a). 
On the other hand, we do not need an exponential protocol for the third term (max) as the term only consists of type-3 distances; we only divide it by $\sigma_{d^2}$ to ensure scale invariance. The resulting formula is as follows:
\begin{align*}
    II_1(C, X, d^2) =\frac{\displaystyle e^{\left(\displaystyle \sum_{x\in X}\frac{d^2(x, c)}{|X|\sigma_{d^2}} \right)}}{|C|\displaystyle e^{\left(\displaystyle \sum_{i=1}^{|C|}\sum_{x\in C_i}\frac{d^2(x, c_i) }{|X| \sigma_{d^2}}\right)}} \max_{1 \leq i, j \leq |C|} \frac{ d^2(c_i, c_j)}{\sigma_{d^2}}.
\end{align*}

\noindent
\textbf{Applying T4 (Range invariance)}
As $\max(II_1) \rightarrow + \infty$, we define $II_2 = 1/(1 + e^{-k \cdot II_1})$ so that $II_{2\max} \rightarrow 1$ (T4-b). As for $CH$ and $DI$, we get $II_3 = (II_2 - II_{2\min}) / (II_{2\max} - II_{2\min})$, where $II_{2\min} = E_{\pi}(II_2(C^{\pi}, X, d^2))$ (T4-a). The $k$ value are set by calibrating $II_3$ using human-judgment separability scores (T4-c).

\noindent
\textbf{Applying T3 (Class-cardinality invariance)} We design $II_A$ to be class-cardinality invariant by averaging class-pairwise scores:
\[
II_A = \frac{1}{{|C| \choose 2}} \sum_{S \subseteq C, |S|=2} II_3(C, X, d).
\]

\noindent
\textbf{Removing Monte-Carlo simulations} As we did for $CH_A$, we can accelerate the computation of $II_A$ by removing Monte-Carlo simulations for estimating $II_{2\min}$. As randomly permuting class labels makes every $C_i \in C$ satisfy $C_i \overset{D}{=} X$, $c \simeq c_i \forall c_i$. Therefore $d^2(c_i, c_j) \simeq 0$, which leads to $II_{1}(C^\pi, X, d^2) \simeq 0$ and $II_{2\min}= E_{\pi}(II_2(C^{\pi}, X, d)) = E_{\pi} (1/2) = 1/2$.

\noindent
\textbf{Computational Complexity}
$II$, $II_1$, $II_2$ is $O(|X|\Delta_X)$, thus $II_{2\min} = O(|X|\Delta_X T)$, where $T$ is the number of Monte Carlo simulations to compute $II_{2\min}$. $II_3$ is thus $O(|X|\Delta_X T)$ and $II_A = O(|X|\Delta_X T |C|)$. Removing the Monte-Carlo simulations reduces the complexity of $II_A$ to $O(|X|\Delta_X |C|)$.

\subsection{Adjusting Xie-Beni index ($XB$)}

Xie-Beni Index \cite{xie91tpami} is defined as:
\[
 XB(C, X, d^2) = \frac{\sum_{i=1}^{|C|}\sum_{x \in C_i}  d^2(x, c_i)}{|X| \cdot \min_{1\leq i, j \leq |C|, i \neq j}d^2(c_i, c_j)}.
\]
$XB$ misses all axioms except data-cardinality invariance. For the adjustment, we first take the inverse formula so that the higher score implies better clustering, resulting in:
\[
XB_1(C, X, d^2) = \frac{|X| \cdot \min_{1\leq i, j \leq |C|, i \neq j}d^2(c_i, c_j)}{\sum_{i=1}^{|C|}\sum_{x \in C_i}  d^2(x, c_i)}
\]

\noindent
\textbf{Applying T2 (Shift invariance)} 
As the denominator consists of type-2 distance while the numerator consists of type-3 distance, we add a factor term with type-2 distances to the numerator to equalize shifting. As we did for $CH$, we add the sum of squared distances of the data points to their centroid. 
We also remove the $|X|$ term from the numerator to ensure the data-cardinality invariance.
This leads to the following:
\[
 XB_2(C, X, d^2) = \frac{\displaystyle \sum_{x \in X} d^2(x, c)}{\displaystyle \sum_{i=1}^{|C|}\sum_{x \in C_i}  d^2(x, c_i)}\cdot \min_{1\leq i, j \leq |C|, i \neq j}d^2(c_i, c_j).
\]
We then apply the exponential protocol (T2-a, b) to the first term, while maintaining the second term as type-3 distances do not shift (we only normalized it by $\sigma_{d^2}$ to ensure scale-invariance). 
{
\small
\begin{align*}
 XB_3(C, X, d^2) = \frac{\exp\left({\displaystyle\sum_{x \in X} \frac{d^2(x, c)}{|X|\sigma_{d^2}}}\right)}{\exp\left({\displaystyle \sum_{i=1}^{|C|}\sum_{x \in C_i} \frac{d^2(x, c_i)}{|X|\sigma_{d^2}}}\right)}\min_{\substack{1\leq i, j \leq |C|\\ i \neq j}}\frac{d^2(c_i, c_j)}{\sigma_{d^2}}.
\end{align*}
}

\sloppy
Here, when we limit $|C|=2$, $XB_3(C, X, d^2) = 2 \cdot II_1 (C, X, d^2)$, as
$\min_{1\leq i, j \leq 2, i \neq j}d^2(c_i, c_j) =\max_{1 \leq i, j \leq 2} d^2(c_i, c_j) = d^2(c_1, c_2) $. 
Therefore, by applying to $XB_3$ the adjustment procedure of $II_1$, we  obtain $XB_A$ which is identical to $II_A$:

$$ \forall C, X, \quad XB_A(C, X, d^2) = II_A(C, X, d^2)$$

\fussy

\subsection{Adjusting Davies-Bouldin Index ($DB$)}

Davies-Bouldin index \cite{davies79tpami} is defined as:
\[
DB(C, X, d) = \frac{1}{|C|} \sum_{i=1}^{|C|} \max_{\substack{1\leq j\leq|C|\\ i \neq j}} \frac{\displaystyle\sum_{k \in \{i, j\}}\frac{1}{|C_k|} \sum_{x \in C_k} d(x, c_k)}{d(c_i, c_j)}.
\]
$DB$ satisfies data-cardinality invariance but misses all other across-dataset axioms. We first inverse the formula, making higher scores imply better clustering (i.e., $DB_1(C, X, d) = DB(C, X, d)^{-1}$).

\noindent
\textbf{Applying T2 (Shift invariance)}
As the denominator use type-3 distances while the numerator consists of type-2 distances, we add an additional term consisting of type-2 distances to the denominator and change the distance function to $d^2$ to equalize shifting. We add the average of squared distances of data points to their centroid, resulting in:
{
\small
\begin{align*}
&DB_2(C, X, d^2) =\left(
\displaystyle\frac{1}{|C|} \sum_{i=1}^{|C|} \max_{\substack{1\leq j\leq|C|\\ i \neq j}} \frac{\displaystyle\sum_{k \in \{i, j\}}\frac{1}{|C_k|}\sum_{x \in C_k} d^2(x, c_k)}{\displaystyle \frac{d^2(c_i, c_j)}{|X|}\sum_{x \in X} d^2(x, c)  
}\right)^{-1} 
\end{align*}
}

We then apply the exponential protocol (T2-a, b) to the first fractional term, while only normalizing the second term with $\sigma_{d^2}$ to ensure  scale invariance:
{
\footnotesize
\begin{align*}
DB_3(C, X, d^2) = 
\left(
\frac{1}{|C|} \sum_{i=1}^{|C|} \max_{\substack{1\leq j\leq|C|\\ i \neq j}}\frac{\displaystyle \sum_{k \in \{i, j\}}e^{\displaystyle  \frac{1}{|C_k|}\sum_{x \in C_k} \frac{d^2(x, c_k)}{\sigma_{d^2}}}} {\displaystyle \frac{d^2(c_i, c_j)}{\sigma_{d^2}} e^{\displaystyle \frac{1}{|X|}\sum_{x \in X} \frac{d^2(x, c)}{  \sigma_{d^2}}}}  
\right)^{-1} 
\end{align*}
}

\noindent
\textbf{Applying T4 (Range invariance)}
We apply min-max scaling to make $DB_A$ range invariant. As $\max(DB_3) \rightarrow +\infty$, we transform the function by applying the logistic function (T4-b), resulting in $DB_4 = 1/(1+e^{-k\cdot DB_3})$, so that $DB_{4\max} \rightarrow 1$. We then get $DB_5 = (DB_4 - DB_{4\min}) / (DB_{4\max} - DB_{4\min})$, where $DB_{4\min} = E^\pi (DB_4(C^\pi, X, d^2)$. $k$ value is calibrated based on human-judgment separability scores (T4-c).

\noindent \sloppy
\textbf{Removing Monte-Carlo simulations}
We remove the Monte-Carlo simulation estimating $DB_{4\min}$ to further accelerate the computation. As randomly permuting class labels makes $C_i \overset{D}{=} X$ $\forall C_i \in C$, thus $c_i \simeq c_j$ and $d^2(c_i, c_j) \simeq 0$ $\forall c_i, c_j$, $DB_3(C^\pi, X, d^2) \simeq 0$, which leads to $DB_{4\min} = E^\pi (DB_4(C^\pi, X, d^2) = E^\pi(1/2) = 1/2$.

\fussy

\noindent
\textbf{Computational Complexity}
The computational complexity of $DB, DB_1, DB_2, DB_3$, and $DB_4$ is $O(|X|\Delta_X)$. Therefore $DB_{4\min} = O(|X|\Delta_X T)$ and $DB_A =  O(|X|\Delta_X T |C|)$ where $T$ is the number of Monte-Carlo simulations to compute $DB_{4\min}$. By removing the simulations, we can reduce the complexity of $DB_A$ to $O(|X|\Delta_X |C|)$.

\subsection{Adjusting the Silhouette Coefficient ($SC$)}

Silhouette Coefficient \cite{rousseeuw87jcam} is defined as:

\[
SC(C, X, d) = \frac{1}{|C|} \cdot \sum_{i=1}^{|C|} \frac{1}{|C_i|}\sum_{x \in C_i} \frac{b(x) - a(x)}{\max(b(x), a(x))}.
\]
For a data point $x \in C_I$, 
\[
a(x) = \frac{1}{|C_I| - 1}\sum_{y \in C_I, x \neq y} d(x, y),
\]
and 
\[
b(x) = \min_{1 \leq J \leq |C|, I \neq J}\frac{1}{|C_J|}\sum_{y \in C_J} d(x, y).
\]
As $SC$ satisfies data-cardinality invariance (A1) and range invariance (A4) (\autorefapp{app:proofs}), we only need to apply the shift (T2) and class-cardinality (T4) protocols.

\noindent
\textbf{Applying T2 (Shift invariance)} As $a(x)$ and $b(x)$ are already robust estimators of population statistics (T1) and also consist of type-1 distances, we simply apply the exponential protocol (T2-a,b) to the terms, resulting in:
\[
SC_1(C, X, d) =  \frac{1}{|C|} \cdot \sum_{i=1}^{|C|} \frac{1}{|C_i|}\sum_{x \in C_i} \frac{b'(x) - a'(x)}{\max(b'(x), a'(x))},
\]
where 
\[
 a'(x) = e^{a(x) / \sigma^{d}} \text{ and } b'(x) = e^{b(x) / \sigma^{d}}.
\]

\noindent
\textbf{Applying T3 (Class-cardinality invariance)} We make $SC_A$ satisfy class-cardinality invariance by averaging class-pairwise scores:
\[
SC_A(C, X, d) = \frac{1}{{|C| \choose 2}} \sum_{S \subseteq C, |S|=2} SC_1(C, X, d).
\]
While $SC$ misses two across-dataset axioms, $SC_A$ satisfies them all.

\noindent
\textbf{Computational Complexity} The complexity of $SC$ and $SC_1$ is $O(|X|^2\Delta_X)$, thus $SC_A = O(|X|^2\Delta_X |C|)$.

\section{Theorems and Proofs}

\label{app:proofs}
% Remind where these theorems ares used in the main paper, which section?

\subsection{About the Shift of Distances}

Here, we prove the theorems about the shift of type-1 and type-2 distances, which form the bases of the equalizing shifting step of the shift protocol (\autoref{sec:tricks} T2-c).

\label{app:proofshift}

\begin{itemize}[leftmargin=0em]
    \setlength\itemsep{4pt}
    
    \item[] 
    \textbf{Theorem 1.} \textit{$\forall X' \subset X$,  $\forall \beta > 0$, and for any Euclidean distance functions $d_L$ and $d_H$ satisfying $d_H^2 = d_L^2 + \beta$, 
   we have $\sum_{x \in X'}d_H^2(x, c) = \sum_{x \in X'}d^2_L(x,c) + \beta/2$, where $c = \overline{X'}$.}
    \item[] 
    \textit{Proof.} According to Hopcroft \& Kannon \cite{hopcroft14foundations}, for any set of data points $X' \subset X$, the following equality holds:
    \[
        2n \cdot \sum_{x \in X'} d^2(x, c)  = \sum_{x \in X'}\sum_{y \in X'} d^2(x,y).
    \]
    Here,
    \begin{align*}
        2n \cdot \sum_{x \in X'} d_H^2(x, c) &= \sum_{x \in X'}\sum_{y \in X'} d^2_H(x,y). \\
                                            &= \sum_{x \in X'}\sum_{y \in X'} (d^2_L + \beta)(x,y) \\
                                            &= n^2\beta + \sum_{x \in X'}\sum_{y \in X'} d^2_L(x,y) \\
                                            &=  n^2\beta + 2n \cdot \sum_{x \in X'} d_L^2(x, c)  \\
                                            &= 2n \cdot \left(\frac{n\beta}{2} + \sum_{x \in X'} d_L^2(x, c) \right) \\
                                            &= 2n \cdot \sum_{x \in X'} \left(d_L^2(x, c) + \frac{\beta}{2}\right)
    \end{align*}
    Therefore, $\sum_{x \in X'}d_H^2(x, c) = \sum_{x \in X'}d^2_L(x,c) + \beta/2$. \hfill $\Box$

    \item[] \textbf{Theorem 2.} \textit{$\forall X', X'' \subset X$, $\forall \beta > 0$, and for any $d_L$ and $d_H$ satisfying $d_H^2 = d_L^2 + \beta$, we have $d^2_H(c', c'') = d^2_L(c', c'')$, where $c' = \overline{X'}$ and $c''= \overline{X''}$.}
    \item[]
    \textit{Proof.} According to Apostol \& Mnatsakanian \cite{apostol03amm}, the following equality holds for any set of points $X'$, $X''$:
    \begin{align*}
        d^2(c_1, c_2) =& \frac{1}{n_{X'}n_{X''}}\sum_{x \in X'}\sum_{y \in X''}d^2(x,y) \\ &- \frac{1}{2n_{X'}^2}\sum_{x \in X'}\sum_{y \in X'}d^2(x,y) \\ &-
        \frac{1}{2n_{X''}^2}\sum_{x \in X''}\sum_{y \in X''}d^2(x,y).
    \end{align*}
    Here, using Theorem 1,
    \begin{align*}
        d^2_H(c_1, c_2) =& \frac{1}{n_{X'}n_{X''}}\sum_{x \in {X'}}\sum_{y\in {X''}}d^2_H(x,y) \\ &- \frac{1}{2n_{X'}^2}\sum_{x \in X'}\sum_{y \in X'}d^2_H(x,y) \\ &-
        \frac{1}{2n_{X''}^2}\sum_{x \in {X''}}\sum_{y \in {X''}}d^2_H(x,y). \\ 
        =& \frac{1}{n_{X'}n_{X''}}\sum_{x \in {X'}}\sum_{y \in {X''}}(d^2_L + \beta)(x,y) \\&- \frac{1}{2n_{X'}^2}\sum_{x \in {X'}}\sum_{y \in {X'}}(d^2_L + \beta)(x,y) \\ &-
        \frac{1}{2n_{X''}^2}\sum_{x \in {X''}}\sum_{y \in {X''}}(d^2_L + \beta)(x,y). \\ 
        =& \frac{1}{n_{X'}n_{X''}}\sum_{x \in {X'}}\sum_{y\in {X''}}d^2_L(x,y) \\ &- \frac{1}{2n_{X'}^2}\sum_{x \in X'}\sum_{y \in X'}d^2_L(x,y) \\ &+ \beta - \beta/2 - \beta/2 -
        \frac{1}{2n_{X''}^2}\sum_{x \in {X''}}\sum_{y \in {X''}}d^2_L(x,y) \\
         =& \frac{1}{n_{X'}n_{X''}}\sum_{x \in {X'}}\sum_{y\in {X''}}d^2_L(x,y) \\ &- \frac{1}{2n_{X'}^2}\sum_{x \in X'}\sum_{y \in X'}d^2_L(x,y) \\ &-
        \frac{1}{2n_{X''}^2}\sum_{x \in {X''}}\sum_{y \in {X''}}d^2_L(x,y)  
        \\ =& d^2_L(c_1, c_2)
    \end{align*}
    
\end{itemize}

% \subsection{About 

\subsection{About Class-Cardinality Invariance}

% We achieve class-cardinality invariance by aggregating local measures class-pairwisely. Here, we prove that if the local measures satisfy the remaining axioms (Shift invariance, range invariance, and data-cardinality invariance), the aggregated global measure also satisfies the axioms.

\label{app:proofclasscard}

\sloppy
Ackerman and Ben-David \cite{bendavid08nips} showed that if a function $f'$ satisfies any of the within-dataset axioms, then its aggregation $f(C, X, \delta)  = \textrm{agg}_{S \subseteq C, |S| = 2} f'(S, X, \delta)$ with $\textrm{agg}\in\{\min,\textrm{avg},\max\}$, also satisfies that axiom, which is represented by the following theorem from \cite{bendavid08nips}: 

\fussy

\begin{itemize}[leftmargin=0em]
    \setlength\itemsep{4pt}
    \item[] \textbf{Theorem 3.} \textit{If $f'$ satisfies a within-dataset axiom, then $\forall \textrm{agg}\in\{\min,\textrm{avg},\max\}, f(C, X, \delta)  = \textrm{agg}_{S \subseteq C, |S| = 2} f'(S, X, \delta)$ also satisfies the axiom.} \cite{bendavid08nips}
\end{itemize}

Here, we use Theorem 3 to prove the same property for across-dataset axioms.

\begin{itemize}[leftmargin=0em]
    \setlength\itemsep{4pt}
    \item[] \textbf{Theorem 4.} \textit{If $f'$ satisfies data-cardinality invariance (A1), then $f(C, X, \delta)  = \textrm{agg}_{S \subseteq C, |S| = 2} f'(S, X, \delta)$ is also data-cardinality invariant.}
    \item[] \sloppy
    \textit{Proof.} At first, $f(C, X, \delta) = \textrm{agg}_{S \subseteq C, |S| = 2} f'(S, X, \delta) $ and $f(\underline{C}_\alpha, X_\alpha, \delta) = \textrm{agg}_{S \subseteq \underline{C}_\alpha, |S| = 2} f'(S, X_\alpha, \delta) $ by definition (A3). Then, as  $\textrm{agg}_{S \subseteq C, |S| = 2} f'(S, X, \delta) = \textrm{agg}_{S \subseteq \underline{C}_\alpha, |S| = 2} f'(S, X_\alpha, \delta)$ (A1), $f(C, X, \delta) = f'(\underline{C}_\alpha, X_\alpha, \delta)$.
    Thus, $f$ satisfies data-cardinality invariance. \hfill $\Box$

    \fussy
    \item[] \sloppy \textbf{Theorem 5.} \textit{If $f'$ satisfies shift invariance, then $f(C, X, \delta)  = \textrm{agg}_{S \subseteq C, |S| = 2} f'(S, X, \delta)$ is also shift-invariant (A2).}
    \item[] \textit{Proof.} By definition (A3), $f(C, X, \delta) = \textrm{agg}_{S \subseteq C, |S| = 2} f'(S, X, \delta)$ and $f(C, X, \delta + \beta) = \textrm{agg}_{S \subseteq C, |S| = 2} f'(S, X, \delta + \beta)$. Then, as $\textrm{agg}_{S \subseteq C, |S| = 2} f'(S, X, \delta) = \textrm{agg}_{S \subseteq C, |S| = 2} f'(S, X, \delta + \beta)$ (A1), $f(C, X, \delta) = f(C, X, \delta + \beta)$. 
    Thus, $f$ satisfies shift invariance.  \hfill $\Box$

    \fussy
    \item[] \textbf{Theorem 6.} \textit{If $f'$ is range invariant over any pair of classes, then $f(C, X, \delta)  = \textrm{agg}_{S \subseteq C, |S| = 2} f'(S, X, \delta)$ is also Range Invariant (A4).}
    \item[] \sloppy \textit{Proof.} Assume $f'$ satisfies Range Invariance; i.e.,

    \[
        \forall S \subseteq C, |S| = 2, f'_{\min}(S,X,\delta)=0 \text{ and } f'_{\max}(S,X,\delta)=1.
    \]
    \fussy
    
     % We want to show that $f_{\min}=\min_C$$(\textrm{agg}_{S \subseteq C, |S| = 2}$$(f'(S,X,\delta)))=0$ and $f_{\max}=\max_C(\textrm{agg}_{S \subseteq C, |S| = 2}(f'(S,X,\delta)))=1$, with $\textrm{agg}\in\{\min,\textrm{avg},\max\}$. \\ 
    From the assumption, we get the following:
    \begin{itemize}[leftmargin=1em]
        \item[](1) $\min_S(f'_{\min})\leq\min_S(f')\leq \min_S(f'_{\max})$ so $\min_S(f')\in[0,1]$
        \item[](2) $\max_S(f'_{\min})\leq\max_S(f')\leq \max_S(f'_{\max})$ so $\max_S(f')\in[0,1]$
        \item[](3)  $\textrm{avg}_S(f'_{\min})\leq\textrm{avg}_S(f')\leq \textrm{avg}_S(f'_{\max})$ so $\textrm{avg}_S(f')\in[0,1]$

    \end{itemize}
    \fussy
    From (1), (2), and (3), we get $\forall C, \forall\textrm{agg}\in\{\min,\textrm{avg},\max\},\\ \textrm{agg}_{S \subseteq C, |S| = 2}(f'(S,X,d))\in[0,1]$
and so $f_{\min}=0$ and $f_{\max}=1$. Thus, $f$ satisfies Range Invariance if $f'$ does so. \hfill $\Box$
    
\end{itemize}

%\textit{Proof.} %Consider $C' = \arg \min_C f'(C, X, d)$ (i.e., $f'(C', X, d) = 0$). Then, for each subset $S$ of $C'$ satisfying $|S|=2$, $f'(S, X, d) = 0$ as $C$ is the worst possible clustering and modifying $C'$ will cause the increment of the score. Therefore, $\min_C f(C, X, d) = f(C', X, d) = \textrm{agg}_{S \subseteq C', |S| = 2} f'(S, X, d) = 0$. 
%In the same way, $\max_C f(C, X, d) = 1$.
%Thus, $f$ is Range Invariance. \hfill $\Box$

\subsection{About Baseline IVMs and Across-Dataset Axioms}

Our main claim is that standard IVM cannot properly evaluate and compare CLM across datasets as they do not satisfy the across-dataset axioms. We provide the proofs verifies the claim.

\subsubsection{About Calinski-Harabasz Index ($CH$)}
\hfill\\

$CH$ \cite{calinski74cis} is defined as:
\[
 CH(C, X, d^2) = \displaystyle\frac{|X| - |C|}{|C| - 1}\cdot\frac{\sum_{i=1}^{|C|}|C_i|d^2(c_i, c)}{\sum_{i=1}^{|C|} \sum_{x \in C_i} d^2(x, c_i)}, 
\]

\begin{itemize}[leftmargin=0em]
    \setlength\itemsep{4pt}

    \item[]
    \textbf{Theorem 7. } \textit{$CH$ does not satisfy data-cardinality invariance (W1). }
    \item[]
    \textit{Proof. }
    In the definition of $CH$, terms $d^2(c_i, c) / (|C| - 1)$ and \\$\sum_{i=1}^{|C|} \sum_{x \in C_i} d^2(x, c_i) / (|X| - |C|)$ are robust estimators of population statistics (average of distances; $|C|$ is the number of classes), thus robust to changes in data cardinality. However, the $|C_i|$ term in the numerator (amount of data in each class) makes $CH$ proportional to the number of points, thus making the function dependent on the data cardinality. \hfill $\Box$
    \item[] 
    \textbf{Theorem 8. } \textit{$CH$ does not satisfy shift invariance (W2). }
    \item[] 
    \textit{Proof. } 
    For any clustering $C$ over $(X, d)$, 
    \begin{align*}
    CH(C, X, d^2 + \beta) &= \frac{|X| - |C|}{|C| - 1}\cdot\frac{|X|\beta+\sum\limits_{i=1}^{|C|}|C_i|d^2(c_i, c)  }{|X|\beta+\sum\limits_{i=1}^{|C|} \sum\limits_{x \in C_i} d^2(x, c_i)} \\ &\neq CH(C, X, d)
    \end{align*}

    $CH$ does not satisfy Shift Invariance.
    \hfill $\Box$
    \item[]
    \textbf{Theorem 9}. \textit{$CH$ does not satisfy class-cardinality invariance (W3).}
    \item[]
    \textit{Proof.} $CH$ does not aggregate scores over pairs of clusters. Its formula cannot be algebraically transformed to an aggregation ($\min,\max,\textrm{avg}$) of cluster-pairwise formula. Therefore, $CH$ does not satisfy class-cardinality invariance by design.   \hfill $\Box$
    \item[] 
    \textbf{Theorem 10.} \textit{$CH$ does not satisfy Range Invariance (W4).}
    \item[]
    \textit{Proof. } The range of $CH$ is $[0, +\infty[$. Therefore, $CH$ is not range invariant as its maximum value is not bounded. \hfill $\Box$
\end{itemize}

\subsubsection{About Dunn Index ($DI$)}

\hfill\\

Dunn Index is defined as 
    \[
    DI(C, X, d) = \frac{\displaystyle \min_{C_i \in C} \min_{C_j \in C, C_i \neq C_j} \min_{x \in C_i, y \in C_j} d(x,y)}{\displaystyle \max_{C_k \in C} \max_{x, y \in C_k, x \neq y} d(x,y)}.
    \]

\begin{itemize}[leftmargin=0em]
    \setlength\itemsep{4pt}

    \item[] 
    \textbf{Theorem 11.} \textit{$DI$ does not satisfy data-cardinality invariance (A1).}

    \item[] 
    \textit{Proof.} 
    $DI$ is a fraction of minimum inter-cluster distances and maximum intra-cluster distances. The minimum and maximum functions are not robust to subsampling, there value can change drastically if the current min or max is not part of the subsample. Thus, $DI$ is not data-cardinality invariant. \hfill $\Box$

    \item[]
    \textbf{Theorem 12. } \textit{$DI$ does not satisfy Shift Invariance (A2).}

    \item[]
    \textit{Proof. } 
    \begin{align*}
    DI(C, X, d + \beta) &= \frac{\beta+\min\limits_{C_i \in C} \min\limits_{\substack{C_j \in C\\ i \neq j}} \min\limits_{\substack{x \in C_i\\ y \in C_j}} d(x,y) }{\beta+\max\limits_{C_k \in C} \max\limits_{\substack{x, y \in C_k\\ x \neq y}} d(x,y)} \\ &\neq DI(C, X, d).
    \end{align*}
    \hfill $\Box$.

    \item[]
    \textbf{Theorem 13. } \textit{$DI$ does not satisfy class-cardinality invariance (A3).}
    
    \item[]
    \textit{Proof.} $DI$ does not aggregate scores over pairs of clusters. Its formula cannot be algebraically transformed to an aggregation ($\min,\max,\textrm{avg}$) of cluster-pairwise formula. Therefore, $DI$ does not satisfy class-cardinality invariance by design. \hfill $\Box$.

    \item[]
    \textbf{Theorem 14. } \textit{$DI$ does not satisfy Range Invariance (A4).} 

    \item[]
    \textit{Proof. } The range of $DI$ is $[0, +\infty[$. Therefore, $DI$ is not range invariant as its maximum value is not bounded. \hfill $\Box$.
    
\end{itemize}

\subsubsection{About I Index ($II$)}

I-Index is defined as 
\[
II(C, X, d) = \left(\frac{1}{|C|} \cdot \frac{\displaystyle \sum_{x\in X}d(x, c)}{\displaystyle \sum_{i=1}^{|C|}\sum_{x\in C_i}d(x, c_i) } \cdot \max_{1 \leq i, j \leq |C|} d(c_i, c_j)\right) ^ p,
\]
\begin{itemize}[leftmargin=0em]
    \setlength\itemsep{4pt}

    \item[]
    \textbf{Theorem 15} \textit{$II$ satisfies data-cardinality invariance (A1).}

    \item[]
    \textit{Proof.} For any $C$ over $(X,d)$,
    %\begin{align*}
    %   II(\underline{C}_\alpha, X_\alpha, d) &= \left(\frac{1}{|C|} \cdot \frac{\sum_{x\in X_\alpha}d(x, c)}{\sum_{i=1}^{|C|}\sum_{x\in \underline{C_i}_\alpha}d(x, c_i) } \cdot \max_{1 \leq i, j \leq |C|} d(c_i, c_j)\right) ^ p \\ 
    %   &=  \left(\frac{1}{|C|} \cdot \frac{\sum_{x\in X}d(x, c) \cdot \alpha}{\sum_{i=1}^{|C|}\sum_{x\in C_i}d(x, c_i) \cdot \alpha} \cdot \max_{1 \leq i, j \leq |C|} d(c_i, c_j)\right) ^ p \\
    %   &= II(C, X, d) 
    %\end{align*}
    II uses averages of distances towards the average (center of gravity) of each class ($c_i$) and of the whole set of points ($c$), and the maximum distance between such centers. Average is a robust estimator of population statistics. Thus, $II$ is data-cardinality invariant.
    \hfill $\Box$

    \item[]
    \textbf{Theorem 16. } 
     \textit{$II$ does not satisfy Shift Invariance (A2).}

    \item[]
    \textit{Proof. } For any $C$ over $(X,d)$,
    \begin{align*}
            II(C, X, d + \beta) &= \left(\frac{1}{|C|} \cdot \frac{|X|\beta+\sum_{x \in X} d(x, c) }{|X|\beta+\sum_{i = 1}^{|C_i|} \sum_{x \in C_i} d(x, c_i)} \right. \\ &\left.\cdot \left(\beta+\max_{_{1 \leq i, j \leq |C|}} d(c_i, c_j)\right)\right)^p 
            \neq II(C, X, d).\\
    \end{align*}
    \hfill $\Box$.

    \item[]
    \textbf{Theorem 17. } \textit{$II$ does not satisfy class-cardinality invariance (A3). }
    \item[]
    \textit{Proof.} $II$ does not aggregate scores over pairs of clusters. Its formula cannot be algebraically transformed to an aggregation ($\min,\max,\textrm{avg}$) of cluster-pairwise formula. Therefore, $II$ does not satisfy class-cardinality invariance by design \hfill $\Box$.
    \item[]
    \textbf{Theorem 18. } \textit{$II$ does not satisfy Range Invariance (A4).} 
    \item[]
    \textit{Proof. } The range of $II$ is $[0, +\infty[$. Therefore, $II$ is not range invariant as its maximum value is not bounded. \hfill $\Box$.
\end{itemize}

\subsubsection{About Xie-Beni Index ($XB$)}
\hfill\\

Xie-Beni Index is defined as:
\[
 XB(C, X, d^2) = \frac{\sum_{i=1}^{|C|}\sum_{x \in C_i}  d^2(x, c_i)}{|X| \min_{1\leq i, j \leq |C|, i \neq j}d^2(c_i, c_j)}.
\]

\begin{itemize}[leftmargin=0em]
    \setlength\itemsep{4pt}

    \item[]
    \textbf{Theorem 19.} \textit{$XB$ satisfies data-cardinality invariance (A1).}

    \item[]
    \textit{Proof.} 
   % For any $C$ over $(X, d)$,
   % \begin{align*}
  %     XB(\underline{C}_\alpha, X_\alpha, d) &= \frac{\sum_{i=1}^{|C|}\sum_{x \in \underline{C_i}_\alpha}  d^2(x, c_i)}{|X_\alpha| \cdot \min_{1\leq i, j \leq |C|, i \neq j}d^2(c_i, c_j) } \\ &= \frac{\sum_{i=1}^{|C|}\sum_{x \in C_i}  d^2(x, c_i) \cdot \alpha}{|X| \cdot \min_{1\leq i, j \leq |C|, i \neq j}d^2(c_i, c_j) \cdot \alpha} \\ &= XB(C, X, d).
  %  \end{align*}
     $XB$ uses averages of distances towards the average (center of gravity) of each class ($c_i$) and the minimum distance between such centers. Averages are robust estimators of population statistics. Thus, $XB$ is data-cardinality invariant. \hfill $\Box$

    \item[]
    \textbf{Theorem 20.} \textit{$XB$ does not satisfy shift invariance (A2).}

    \item[]
    \textit{Proof.}
    For any $C$ over $(X, d)$,
    \begin{align*}
        XB(C, X, d^2 + \beta) &= \frac{|X|\beta+\sum_{i=1}^{|C|}\sum_{x \in C_i} d^2(x, c_i) }{|X| \left(\beta+ \min\limits_{1\leq i, j \leq |C|, i \neq j} d^2(c_i, c_j)\right) } \\ &\neq XB(C, X, d^2).
    \end{align*}
    Thus, $XB$ does not satisfy Shift Invariance. \hfill $\Box$

    \item[]
    \textbf{Theorem 21.} \textit{$XB$ does not satisfy class-cardinality invariance (A3).}

    \item[]
    \textit{Proof. } $XB$ does not aggregate scores over pairs of clusters. Its formula cannot be algebraically transformed to an aggregation ($\min,\max,\textrm{avg}$) of cluster-pairwise formula. Therefore, $XB$ does not satisfy class-cardinality invariance by design. \hfill $\Box$.

    \item[]
    \textbf{Theorem 22. }\textit{$XB$ does not satisfy Range Invariance (A4). }

    \item[]
    \textit{Proof.}  The range of $XB$ is $[0, +\infty[$. Therefore, $XB$ is not range invariant as its maximum value is not bounded. \hfill $\Box$.
\end{itemize}

\subsubsection{About Davies-Bouldin Index ($DB$)}

\hfill\\
Davies-Bouldin index is defined as:
\[
DB(C, X, d) = \frac{1}{|C|} \displaystyle\sum_{i=1}^{|C|} \max_{1 \leq j \leq |C|, i \neq j} \frac{\displaystyle \sum_{k \in \{i, j\}}\frac{1}{|C_k|} \sum_{x \in C_k} d(x, c_k)}{d(c_i, c_j)}.
\]

\begin{itemize}[leftmargin=0em]
    \setlength\itemsep{4pt}

    \item[]
    \textbf{Theorem 23.} \textit{$DB$ satisfies data-cardinality invariance (A1).}

    \item[]
    \textit{Proof.}
    %For any $C$ over $(X, d)$,
    %\begin{align*}
    %    DB(\underline{C}_\alpha, X_\alpha, d) &= \frac{1}{|C|} \sum_{i=1}^{|C|} \max_{1 \leq j \leq |C|, i \neq j} \frac{\sum_{k \in \{i, j\}}\frac{1}{|\underline{C_k}_\alpha|} \sum_{x \in \underline{C_k}_\alpha} d(x, c_k)}{d(c_i, c_j)} \\ &= \frac{1}{|C|} \sum_{i=1}^{|C|} \max_{1 \leq j \leq |C|, i \neq j} \frac{\sum\limits_{k \in \{i, j\}}\frac{1}{|C_k| \cdot \alpha} \sum_{x \in C_k} d(x, c_k) \cdot \alpha}{d(c_i, c_j)}    
    %    \\ &= DB(C, X, d).
    %\end{align*}
     $DB$ uses averages of distances towards the average (center of gravity) of each class ($c_i$) and the minimum distance between such centers. Averages are robust estimators of population statistics. Thus, $DB$ satisfies data-cardinality invariance. \hfill $\Box$

    \item[]
    \textbf{Theorem 24.} \textit{$DB$ does not satisfy shift invariance (A2).}
    For any $C$ over $(X,d)$,
    {
    \small
    \begin{align*}
        &DB(C, X, d + \beta)\\  &= \frac{1}{|C|} \sum_{i=1}^{|C|} \max_{\substack{j \in \{1,\cdots,|C|\}\\ i \neq j}} \frac{\frac{1}{|C_i|} \sum\limits_{x \in C_i} d(x, c_i) + \frac{1}{|C_j|} \sum\limits_{x \in C_j} d(x, c_j) + 2\beta}{d(c_i, c_j) + \beta} \\ 
  &\neq DB(C, X, d).
    \end{align*}
    }
    Thus, $DB$ does not satisfy shift invariance.

    \item[]
    \textbf{Theorem 25.} \textit{$DB$ does not satisfy class-cardinality invariance (A3).}

    \item[]
    \textit{Proof.} $DB$ does not aggregate scores over pairs of clusters. Its formula cannot be algebraically transformed to an aggregation ($\min,\max,\textrm{avg}$) of cluster-pairwise formula. Therefore, $DB$ does not satisfy class-cardinality invariance by design. \hfill $\Box$

    \item[]
    \textbf{Theorem 26. }\textit{$DB$ does not satisfy Range Invariance (A4). }

    \item[]
    \textit{Proof. }  The range of $DB$ is $[0, +\infty[$. Therefore, $DB$ is not range invariant as its maximum value is not bounded. \hfill $\Box$.
\end{itemize}

\subsubsection{About Silhouette Coefficient ($SC$)}

\hfill\\
Silhouette Coefficient is defined as:

\[
SC(C, X, d) = \frac{1}{|C|} \cdot \sum_{i=1}^{|C|} \frac{1}{|C_i|}\sum_{x \in C_i} \frac{b(x) - a(x)}{\max(b(x), a(x))}.
\]
For a data point $x \in C_I$, 
\[
a(x) = \frac{1}{|C_I| - 1}\sum_{y \in C_I, x \neq y} d(x, y),
\]
and 
\[
b(x) = \min_{1 \leq J \leq |C|, I \neq J}\frac{1}{|C_J|}\sum_{y \in C_J} d(x, y).
\]
\begin{itemize}[leftmargin=0em]
    \setlength\itemsep{4pt}

    \item[]
    \textbf{Theorem 27.} \textit{$SC$ satisfies data-cardinality invariance (A1).}

    \item[]
    \textit{Proof.} $a(x)$ and $b(x)$, two building blocks of $SC$, are both robust estimators of population statistics (average distances), and thus are data-cardinality invariance. Therefore, $SC$ is data-cardinality invariance.

    \item[]
    \textbf{Theorem 28.} \textit{$SC$ does not satisfy shift invariance (A2).}

    \item[]
    \textit{Proof.} For any $C$ over $(X, d)$,
    \begin{align*}
        SC(C, X, d + \beta) &= \frac{1}{|C|} \cdot \sum_{i=1}^{|C|} \frac{1}{|C_i|}\sum_{x \in C_i} \frac{b(x) - a(x)}{\beta + \max(b(x), a(x))} \\ &\neq SC(C,X, d).
    \end{align*}

    Thus, $SC$ is not shift invariant. \hfill $\Box$

    \item[]
    \textbf{Theorem 29.} \textit{$SC$ does not satisfy class-cardinality Invariance (A3).}

    \item[]
    \textit{Proof.} $SC$ does not aggregate scores over pairs of clusters. Its formula cannot be algebraically transformed to an aggregation ($\min,\max,\textrm{avg}$) of cluster-pairwise formula. Therefore, $SC$ does not satisfy class-cardinality invariance by design. \hfill $\Box$

    \item[]
    \textbf{Theorem 30. }\textit{$SC$ satisfies Range Invariance (A4). }

    \item[]
    \textit{Proof.} The theoretical range of $SC$ is $[-1, 1]$, and the expected minimum of the measure (based on randomly permuted class labels) is 0. Therefore, $SC$ is range invariant.

\end{itemize}

\subsection{About $CH_A$ and Across-Dataset Axioms}

\begin{itemize}[leftmargin=0em]
    \setlength\itemsep{4pt}

        \item[]
    \textbf{Theorem 31.} $CH_5$ satisfies data-cardinality invariance (A1).

    \item[]
    \textit{Proof.}
    $CH_A$ uses averages of distances towards the center of gravity of each class ($c_i$) or the entire dataset ($c$), or the average of distances between the centers. Averages are robust estimators of population statistics. Thus, $CH_5$ satisfies data-cardinality invariance. Due to Theorem 4, $CH_A$ is also data-cardinality invariant as it is the class-pairwise aggregation of $CH_5$.
    
    \hfill $\Box$

    \item[]
    \textbf{Theorem 32.} $CH_A$ satisfies shift invariance (A2).

    \item[]
    \textit{Proof.} For any $C$ over $(X, d)$,
    {
    \small
    \begin{align*}
        CH_{3}(C, X, d^2 + \beta) &= \displaystyle\frac{e^{\frac{\sum\limits_{x \in X} (d^2(x, c) + \beta)}{\sigma_{d^2} \cdot |X|}}}{e^{\frac{\sum\limits_{i=1}^{|C|} \sum\limits_{x \in C_i} (d^2(x, c_i)+\beta)}{ \sigma_{d^2} \cdot|X|}}} \cdot \frac{\sum\limits_{i=1}^{|C|}|C_i|(d^2(c_i, c) + \beta)}{\sigma_{d^2} \cdot|X| \cdot (|C| - 1)} \\
        &= \displaystyle\frac{e^{\frac{\sum\limits_{x \in X} d^2(x, c)}{\sigma_{d^2} \cdot |X|}} e^{\frac{\beta}{\sigma_{d^2}}}}{e^{\frac{\sum\limits_{i=1}^{|C|} \sum\limits_{x \in C_i} d^2(x, c_i)}{ \sigma_{d^2} \cdot|X|}}e^{\frac{\beta}{\sigma_{d^2}}}} \cdot \frac{\sum\limits_{i=1}^{|C|}|C_i|d^2(c_i, c)}{\sigma_{d^2} \cdot|X| \cdot (|C| - 1)} \\
        &= CH_3(C,X, d^2).
    \end{align*}
    }
    Therefore, $CH_3$ is shift invariant, thus $CH_4$ and $CH_5$ are also shift invariant. Due to Theorem 5, $CH_A$ is also shift invariant as it is the class-pairwise aggregation of $CH_5$. 
    \hfill $\Box$

    \item[]
    \textbf{Theorem 33.} $CH_A$ satisfies class-cardinality invariance (A3).

    \item[]
    \textit{Proof.} $CH_A$ is defined as the class-pairwise aggregation of $CH_5$, thus is class-cardinality invariant \hfill $\Box$.

    \item[]
    \textbf{Theorem 34.} $CH_A$ satisfies range invariance (A4)

    \item[]
    \textit{Proof.} The range of $CH_5$ is $[0,1]$. thus $CH_5$ is range invariant. Therefore, due to Theorem 6, $CH_A$ is also range invariant as it is the class-pairwise aggregation of $CH_5$. \hfill $\Box$

\end{itemize}

\section{Base Gaussian Datasets}

For the ablation study (\autoref{sec:validity}) and logistic growth rate calibration (\autoref{sec:trick4} T4-c), we used datasets where each consisting of two Gaussian clusters with diverse hyperparameters. \autoref{fig:basis} shows a subset of 28 scatterplot representations of these datasets among 1000 available.

\begin{figure}[t]
    \centering
    \includegraphics[width=\linewidth]{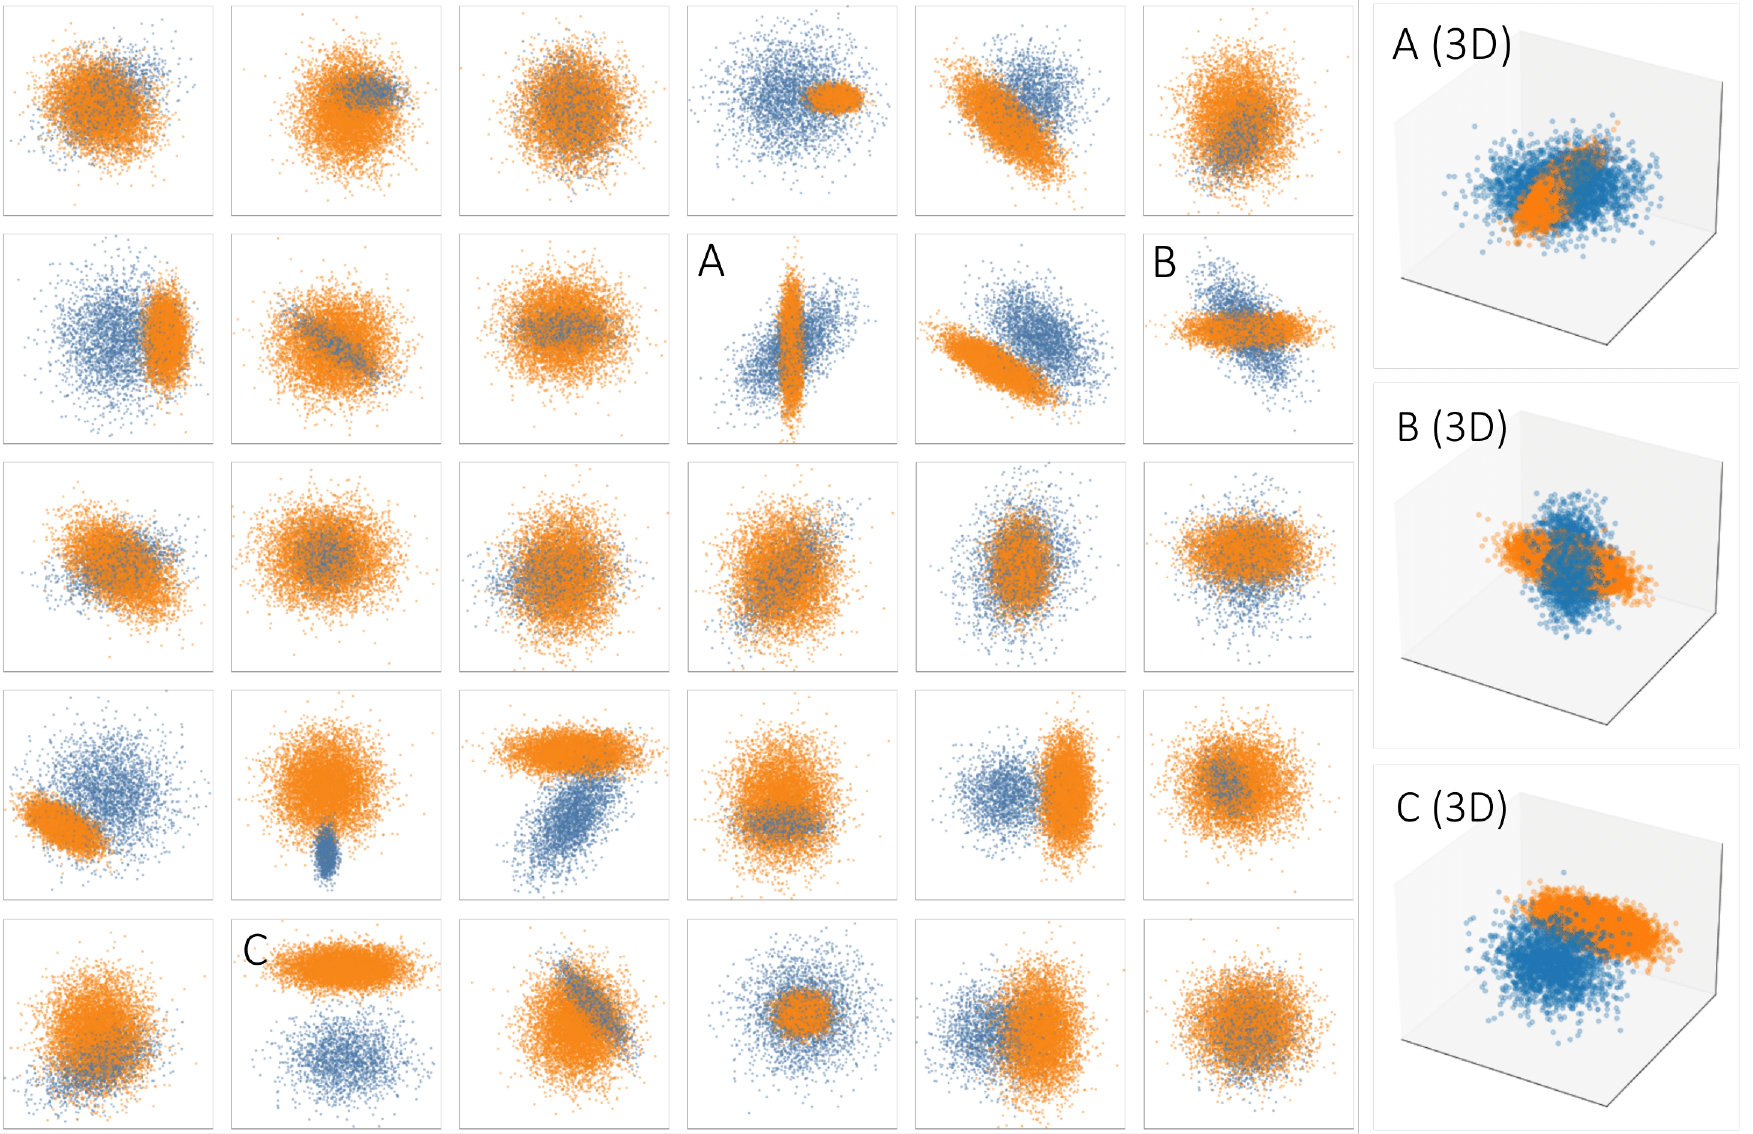}
    \vspace{-5mm}
    \caption{Subset of 1,000 base datasets used in the ablation study (\autoref{sec:validity})  and logistic growth rate calibration (\autoref{sec:trick4} T4-c); we displayed the first two (left) and three (right) axes of each dataset. Note that only the first two axes are used to calibrate the logistic growth rate of \IVMa.
    }
    \label{fig:basis}
\end{figure}

\section{Experimental Setting}

\label{app:setting}

\noindent
\textbf{Classifiers settings } As aforementioned in Section 5.2., we exploited Bayesian Optimization \cite{snoek12neurips} to find the best hyperparameter setting of the classifiers for each fold of cross validation. We used the implementation of Nogueira \cite{nogueira14github}. For each classifiers, we performed five random exploration and 25 steps of optimization, following the default setting of the implementation. For the bounds of the hyperparameters, we exploited the settings provided by \texttt{auto-sklearn} \cite{feurer15nips}. For the hyperparameters that are not mentioned below, we used the default provided by \texttt{sklearn}. 
\begin{itemize}
    \item \textbf{Support Vector Machine} (SVM)
    \begin{itemize}
        \item \texttt{C}: [$2^{-5}, 2^{5}$]
        \item \texttt{gamma}: [$2^{-15}, 2^3$]
    \end{itemize}
    \item \textbf{$k$-Nearest Neighbor} ($k$NN)
    \begin{itemize}
        \item \texttt{n\_neighbors}: [1, $2 \cdot \sqrt{\text{|X|}}$], where $|X|$ denotes the number of data points
    \end{itemize}
    \item \textbf{Multilayer Perceptron} (MLP)
    \begin{itemize}
        \item \texttt{hidden\_layer\_depth}: [1, 4]
        \item \texttt{num\_nodes\_per\_layer}: [16, 256]
        \item \texttt{activation}: \{\texttt{identity}, \texttt{logistic}, \texttt{tanh}, \texttt{relu}\}
        \item \texttt{alpha}: [$10^{-7}, 10^{-1}$]
        \item \texttt{learning\_rate\_init}: [$10^{-4}$, 0.5]
    \end{itemize}
    \item \textbf{Naive Bayesian networks} (NB)
    \begin{itemize}
        \item \texttt{var\_smoothing}: [$10^{-12}, 1$]
    \end{itemize}
    \item \textbf{Random forest} (RF)
    \begin{itemize}
        \item \texttt{n\_estimators}: [1, 200]
        \item \texttt{min\_samples\_split}: [2, 20]
        \item \texttt{min\_samples\_leaf}: [1, 20],
        \item \texttt{criterion}: \{\texttt{gini}, \texttt{entropy}, \texttt{log\_loss}\}
    \end{itemize}
    \item \textbf{Logistic regression} (LR)
    \begin{itemize}
        \item \texttt{penalty}: \{\texttt{L1}, \texttt{L2}, \texttt{Elasticnet}\}
        \item \texttt{C}: [$2^{-5}, 2^{5}$]
        \item \texttt{tol}: [$10^{-5}, 10^{-1}$]
        \item \texttt{l1\_ratio}: [0, 1]
    \end{itemize}
    \item \textbf{Linear discriminant analysis} (LDA)
    \begin{itemize}
        \item \texttt{tol}: [$10^{-5}, 10^{-1}$]
        \item \texttt{solver}: \{\texttt{svd}\}
    \end{itemize}
\end{itemize}

For the ensemble of classifiers, we used the max combination of the classifiers (i.e., chose the highest score among the classifiers). Finally, we estimated the CLM ranking of the labeled datasets based on the classification scores.

\noindent
\textbf{Settings for computing ground-truth CLM.}
We used \texttt{sklearn} implementation for DBSCAN, $K$-Means, Birch, Agglomerative clustering, and used \texttt{sklearn-extra} implementation for $K$-Medoids. We used \texttt{pyclustering} implementation for $X$-Means. For HDBSCAN, we used the implementation of McInnes et al. \cite{mcinnes17oss}. 
To find the best hyperparameter setting for each clustering technique, we used Nogueira's Bayesian optimization implementation \cite{nogueira14github} with default setting, as we did for classification techniques. 
The bounds of each technique's hyperparameter is set as follows:
\begin{itemize}
    \item \textbf{DBSCAN}
    \begin{itemize}
        \item \texttt{epsilon}: [0.01, 1.0]
        \item \texttt{min\_samples}: [1, 10]
    \end{itemize}
    \item \textbf{HDBSCAN}
    \begin{itemize}
        \item \texttt{epsilon}: [0.01, 1.0]
        \item \texttt{min\_samples}: [1, 10]
        \item \texttt{min\_cluster\_size}: [2, 50]
    \end{itemize}
    \item \textbf{\textit{K}-Means}
    \begin{itemize}
        \item $K$ (number of clusters): [2, $|C| \cdot$ 3], where $|C|$ denotes the number of classes in data
    \end{itemize}
    \item \textbf{\textit{K}-Medoids}
    \begin{itemize}
        \item $K$: [2,  $ |C| \cdot$ 3]
    \end{itemize}
    \item \textbf{\textit{X}-Means}
    \begin{itemize}
        \item \texttt{kmax}: [2, 50]
        \item \texttt{tolerance}: [0.01, 1.0]
    \end{itemize}
    \item \textbf{Birch}
    \begin{itemize}
        \item \texttt{threshold}: [0.1, 1.0]
        \item \texttt{branching\_factor}: [10, 100]
    \end{itemize}
    \item \textbf{Agglomerative Clustering}
    \begin{itemize}
        \item number of clusters: [2, $ |C| \cdot$ 3]
    \end{itemize}
\end{itemize}

We used Single, Average, and Complete variants of Agglomerative Clustering. After finding the best hyperparameter setting of a clustering technique for a given datasets, we ran the technique 20 times with the same setting and report the average value as the final score.

\section{Labeled Datasets}

\label{app:datasets}

Please refer to the end of this document for the tables  containing the list of labeled datasets used in our across-dataset rank correlation analysis (Section 5.2; \autoref{tab:dataset-table} and \ref{tab:dataset2-table}). Note that before applying the clustering techniques, classifiers, and measures, we normalized the datasets and removed the rows containing missing data.

% \newpage

\begin{table*}[t]
    
  \caption{96 Labeled datasets used in across-dataset rank correlation analysis 
 (Ordered by source frequency then alphabetically)}
  \label{tab:dataset-table}
  \centering \small
  \begin{tabular}{lllll}
    \toprule
    Dataset & Objects & Features & Classes & Source \\
    \midrule
        Birds Bones and Living Habits & 413 & 10 & 6 & Kaggle ~\cite{kaggle2022} \\
        Cardiovascular Study & 2,927 & 15 & 2 & Kaggle \\
        Credit Risk Classification & 976 & 11 & 2 & Kaggle \\
        Customer Classification & 1,000 & 11 & 4 & Kaggle \\
        Fraud Detection Bank  & 20,468 & 112 & 2 & Kaggle \\
        Heart Attack Analysis \& Prediction & 303 & 13 & 2 & Kaggle \\
        % League of Legends Diamond Games & 48,651 & 17 & 2 & Kaggle \\
        Microbes & 30,527 & 24 & 10 & Kaggle \\
        Mobile Price Classification & 2,000 & 20 & 4 & Kaggle \\
        Music Genre Classification & 1,000 & 26 & 10 & Kaggle \\
        Orbit Classification For Prediction / NASA & 1,748 & 11 & 6 & Kaggle \\ % Orbit NASA
        Paris Housing Classification & 10,000 & 17 & 2 & Kaggle \\
        Predicting Pulsar Star & 9273 & 8 & 2 & Kaggle \\
        pH-recognition & 653 & 3 & 15 & Kaggle \\
        Rice Seed (Gonen\&Jasmine) & 18,185 & 10 & 2 & Kaggle \\ % Rice type classification
        Siberian Weather Stats & 1,439 & 11 & 9 & Kaggle \\
        Smoker Condition & 1,012 & 7 & 2 & Kaggle \\
        Water Quality & 2,011 & 9 & 2 & Kaggle \\
        Wine Customer Segmentation & 178 & 13 & 3 & Kaggle \\ % Wine Customer
        
        Banknote Authentication & 1,372 & 4 & 2 & UCI ML Repo~\cite{asuncion07uci} \\
        Breast Cancer Wisconsin (Prognostic) & 569 & 30 & 2 & UCI ML Repo \\
        Breast Tissue & 106 & 9 & 6 & UCI ML Repo \\
        CNAE-9 & 1,080 & 856 & 9 & UCI ML Repo \\
        Dermatology & 358 & 34 & 6 & UCI ML Repo \\
        Echocardiogram & 61 & 10 & 2 & UCI ML Repo \\
        Ecoli & 336 & 7 & 8 & UCI ML Repo \\
        Glass Identification & 214 & 9 & 6 & UCI ML Repo \\
        Harberman's Survival & 306 & 3 & 2 & UCI ML Repo \\
        Hepatitis & 80 & 19 & 2 & UCI ML Repo \\
        Image Segmentation & 210 & 19 & 7 & UCI ML Repo \\
        Ionosphere & 351 & 34 & 2 & UCI ML Repo \\
        Iris & 150 & 4 & 3 & UCI ML Repo \\
        Letter Recognition & 20,000 & 16 & 26 & UCI ML Repo \\
        MAGIC Gamma Telescope & 19,020 & 10 & 2 & UCI ML Repo \\
        Optical Recognition of Handwritten Digits & 3,823 & 64 & 10 & UCI ML Repo \\
        Pen-Based Recognition of Handwritten Digits & 7,494 & 16 & 10 & UCI ML Repo \\
        Planning Relax & 182 & 12 & 2 & UCI ML Repo \\
        SECOM & 1,567 & 590 & 2 & UCI ML Repo \\ % secom
        Spambase & 4,601 & 57 & 2 & UCI ML Repo \\
        SPECTF Heart & 80 & 44 & 2 & UCI ML Repo \\
        Statlog (German Credit) & 1,000 & 24 & 2 & UCI ML Repo \\ % German Credit Numeric
        Statlog (Image Segmentation) & 2,310 & 19 & 7 & UCI ML Repo \\
        Taiwanese Bankruptcy Prediction & 6,819 & 95 & 2 & UCI ML Repo \\ % Company Bankruptcy Prediction
        Wine & 178 & 13 & 3 & UCI ML Repo \\
        Yeast & 1,484 & 8 & 10 & UCI ML Repo \\
        Zoo & 101 & 16 & 7 & UCI ML Repo \\
        
        Blood Transfusion Service Center & 748 & 4 & 2 & Yeh et al.~\cite{yeh2009knowledge} \\
        Boston & 154 & 13 & 3 & Sedlmair et al.~\cite{sedlmair2012taxonomy} \\
        Breast Cancer Coimbra & 116 & 9 & 2 & Patrício et al.~\cite{patricio2018using} \\
        Breast Cancer Wisconsin (Original) & 683 & 9 & 2 & Wolberg et al.~\cite{wolberg1990multisurface} \\
        CIFAR10 & 3,250 & 1,024 & 10 & Krizhevsky et al.~\cite{krizhevsky2009learning} \\ % cifar10
        Classification in Asteroseismology & 1,001 & 3 & 2 & Hon et al.~\cite{hon2017deep} \\
        COIL20 & 1,440 & 400 & 20 & Nene et al.~\cite{nene20columbia} \\ % coil20
        Crowdsourced Mapping & 10,545 & 28 & 6 & Johnson et al.~\cite{johnson2016integrating} \\
         Date Fruit & 898 & 34 & 7 & Koklu et al.~\cite{koklu2021classification} \\
        Diabetic Retinopathy Debrecen & 1,151 & 19 & 2 & Antal et al.~\cite{antal2014ensemble} \\
        Dry Bean& 13,611 & 16 & 7 & Koklu et al.~\cite{koklu2020multiclass} \\
    \bottomrule
    
  \end{tabular}
  
\end{table*}

\begin{table*}[t]
  \label{dataset-table2}
  \centering \small
  \begin{tabular}{lllll}
    \toprule
    Dataset & Objects & Features & Classes & Source \\
    \midrule
       
        Durum Wheat Features & 9,000 & 236 & 3 & Kaya et al.~\cite{kaya2019towards} \\
        Epileptic Seizure Recognition & 5,750 & 178 & 5 & Andrzejak et al.~\cite{andrzejak2001indications} \\ % epileptic
        ExtyaleB & 319 & 30 & 5 & Georghiades et al.~\cite{georghiades2001few} \\
        Fashion-MNIST & 3,000 & 784 & 10 & Xiao et al.~\cite{xiao2017fashion} \\ % fashion mnist
        Fetal Health Classification & 2,126 & 21 & 3 & Ayres-de-Campos et al.~\cite{ayres2000sisporto} \\
        Flickr Material Database & 997 & 1,536 & 10 & Sharan et al.~\cite{sharan2009material} \\ % fmd
        HAR & 735 & 561 & 6 & Anguita et al.~\cite{anguita2012human} \\ % har
        Hate Speech & 3,221 & 100 & 3 & Davidson et al.~\cite{davidson2017automated} \\ % hatespeech
        Heart Disease & 297 & 13 & 5 & Detrano et al.~\cite{detrano1989international} \\
        HIVA & 3,076 & 1,617 & 2 & Guyon et al.~\cite{guyon2007agnostic} \\ % hiva
        HTRU2 & 17,898 & 8 & 2 & Lyon et al.~\cite{lyon2016fifty} \\ % Pulsar Dataset HTRU2
        Human Stress Detection & 2,001 & 3 & 3 & Rachakonda et al.~\cite{rachakonda2019stress} \\ % Stress Detection
        IMDB & 3,250 & 700 & 2 & Maas et al.~\cite{maas2011learning} \\ % imdb
        Insurance Company Benchmark  & 5,822 & 85 & 2 & Putten et al.~\cite{van2004bias} \\ % The Insurance Company (TIC) Benchmark
        Labeled Faces in the Wild & 2,200 & 5,828 & 2 & Huang et al.~\cite{huang2008labeled} \\
        Mammographic Mass & 830 & 5 & 2 & Elter et al.~\cite{elter2007prediction} \\
        MNIST64 & 1,082 & 64 & 6 &  Xia et al.~\cite{xia22tvcg} \\
        Olivetti Faces & 400 & 4,096 & 40 & AT\&T Lab. Cambridge~\cite{atntlab} \\
        Parkinsons & 195 & 22 & 2 & Little et al.~\cite{little2007exploiting} \\ % Parkinsons Disease Dataset
        Patient Treatment Classification & 4,412 & 10 & 2 & Mujiono Sadikin~\cite{sadikin2020} \\
        Pima Indians Diabetes Database & 768 & 8 & 2 & Smith et al.~\cite{smith1988using} \\
        Pistachio & 2,148 & 28 & 2 & Ozkan et al.~\cite{ozkan2021classification} \\
        Pumpkin Seeds  & 2,500 & 12 & 2 & Koklu et al.~\cite{koklu2021use} \\
        Raisin & 900 & 7 & 2 & Cinar et al.~\cite{ccinar2020classification} \\
        Rice Dataset Cammeo and Osmancik & 3,810 & 7 & 2 & Cinar et al.~\cite{cinar2019classification} \\
        Seeds & 210 & 7 & 3 & Charytanowicz et al.~\cite{charytanowicz2010complete} \\
        Seismic Bumps & 646 & 24 & 2 & Sikora et al.~\cite{sikora2010application} \\ % seismic
        Sentiment Labeled Sentences & 2,748 & 200 & 2 & Kotzias et al.~\cite{kotzias2015group} \\ % sentiment
        SkillCraft1 Master Table Dataset & 3,338 & 18 & 7 & Thompson et al.~\cite{thompson2013video} \\ % SkillCraft-StarCraft
        SMS Spam Collection & 835 & 500 & 2 & Almeida et al.~\cite{almeida2011contributions} \\ % sms
        Street View House Numbers & 732 & 1,024 & 10 & Netzer et al.~\cite{netzer2011reading} \\ % svhn
        Student Grade & 395 & 29 & 2 & Cortez et al.~\cite{cortez2008using} \\
        Turkish Music Emotion  & 400 & 50 & 4 & Er et al.~\cite{er2019music} \\
        User Knowledge Modeling & 258 & 5 & 4 & Kahraman et al.~\cite{kahraman2013development} \\
        Weather & 365 & 192 & 7 & Ventocilla et al.~\cite{ventocilla2020comparative} \\
        Website Phishing & 1,353 & 9 & 3 & Abdelhamid et al.~\cite{abdelhamid2014phishing} \\
        Wilt & 4,339 & 5 & 2 & Johnson et al.~\cite{johnson2013hybrid} \\
        Wine Quality & 4,898 & 11 & 7 & Cortez et al.~\cite{cortez2009modeling} \\
        Wireless Indoor Localization & 2,000 & 7 & 4 & Rohra et al.~\cite{rohra2017user} \\
        World12d & 150 & 12 & 5 & Sedlmair et al.~\cite{sedlmair2012taxonomy} \\
    \bottomrule
    
  \end{tabular}
  
\end{table*}

\begin{table*}[t]
    
  \caption{96 Labeled datasets ordered by $CH_{A}$ score. The top and bottom 32 datasets (\texttt{top-1/3}  $\mathcal{P}^+$ and \texttt{bottom-1/3}  $\mathcal{P}^-$, respectively, in \autoref{sec:selection}) are  separated by double horizontal lines.}
  \label{tab:dataset2-table}
  \centering \small
  \begin{tabular}{lllll}
    \toprule
    Dataset & Objects & Features & Classes & $CH_{A}$ \\
    \midrule
        Weather & 365 & 192 & 7 & 1.000 \\
        Olivetti Faces & 400 & 4,096 & 40 & 0.956 \\
        MNIST64 & 1,082 & 64 & 6 & 0.956 \\
        Optical Recognition of Handwritten Digits & 3,823 & 64 & 10 & 0.941 \\
        Seeds & 210 & 7 & 3 & 0.925 \\
        Wireless Indoor Localization & 2,000 & 7 & 4 & 0.915 \\
        COIL20 & 1,440 & 400 & 20 & 0.887 \\ % coil20
        Iris & 150 & 4 & 3 & 0.875 \\
        Pen-Based Recognition of Handwritten Digits & 7,494 & 16 & 10 & 0.862 \\
        Rice Seed (Gonen\&Jasmine) & 18,185 & 10 & 2 & 0.861 \\ % Rice type classification
        Breast Cancer Wisconsin (Original) & 683 & 9 & 2 & 0.800 \\
        pH-recognition & 653 & 3 & 15 & 0.780 \\
        Echocardiogram & 61 & 10 & 2 & 0.770 \\
        Fashion-MNIST & 3,000 & 784 & 10 & 0.739 \\ % fashion mnist
        Mobile Price Classification & 2,000 & 20 & 4 & 0.732 \\
        Human Stress Detection & 2,001 & 3 & 3 & 0.722 \\ % Stress Detection
        Dry Bean & 13,611 & 16 & 7 & 0.694 \\
        HAR & 735 & 561 & 6 & 0.690 \\ % har
        Rice Dataset Cammeo and Osmancik & 3,810 & 7 & 2 & 0.654 \\
        Wine Customer Segmentation & 178 & 13 & 3 & 0.619 \\ % Wine Customer
        Wine & 178 & 13 & 3 & 0.619 \\
        Zoo & 101 & 16 & 7 & 0.605 \\
        Image Segmentation & 210 & 19 & 7 & 0.576 \\
        Boston & 154 & 13 & 3 & 0.574 \\
        Statlog (Image Segmentation) & 2,310 & 19 & 7 & 0.514 \\
        Letter Recognition & 20,000 & 16 & 26 & 0.511 \\
        User Knowledge Modeling & 258 & 5 & 4 & 0.485 \\
        Ecoli & 336 & 7 & 8 & 0.472 \\
        Website Phishing & 1,353 & 9 & 3 & 0.407 \\
        Date Fruit & 898 & 34 & 7 & 0.372 \\
        Music Genre Classification & 1,000 & 26 & 10 & 0.340 \\
        Pistachio & 2,148 & 28 & 2 & 0.308 \\
        \midrule
        \midrule
        Crowdsourced Mapping & 10,545 & 28 & 6 & 0.297 \\
        Raisin & 900 & 7 & 2 & 0.294 \\
        Breast Cancer Wisconsin (Prognostic) & 569 & 30 & 2 & 0.294 \\
        Yeast & 1,484 & 8 & 10 & 0.269 \\
        Dermatology & 358 & 34 & 6 & 0.254 \\
        Glass Identification & 214 & 9 & 6 & 0.253 \\
        Classification in Asteroseismology & 1,001 & 3 & 2 & 0.249 \\
        Breast Tissue & 106 & 9 & 6 & 0.216 \\
        Mammographic Mass & 830 & 5 & 2 & 0.202 \\
        Banknote Authentication & 1,372 & 4 & 2 & 0.197 \\
        Birds Bones and Living Habits & 413 & 10 & 6 & 0.186 \\
        ExtyaleB & 319 & 30 & 5 & 0.148 \\
        Flickr Material Database & 997 & 1,536 & 10 & 0.137 \\ % fmd
        CNAE-9 & 1,080 & 856 & 9 & 0.130 \\
        Fetal Health Classification & 2,126 & 21 & 3 & 0.126 \\
        Durum Wheat Features & 9,000 & 236 & 3 & 0.121 \\
        Smoker Condition & 1,012 & 7 & 2 & 0.104 \\
        Student Grade & 395 & 29 & 2 & 0.098 \\
        Turkish Music Emotion  & 400 & 50 & 4 & 0.097 \\
        CIFAR10 & 3,250 & 1,024 & 10 & 0.070 \\ % cifar10
        Ionosphere & 351 & 34 & 2 & 0.069 \\
        SPECTF Heart & 80 & 44 & 2 & 0.066 \\
        Microbes & 30,527 & 24 & 10 & 0.050 \\
        Hate Speech & 3,221 & 100 & 3 & 0.045 \\ % hatespeech
        Predicting Pulsar Star & 9273 & 8 & 2 & 0.033 \\
    \bottomrule
  \end{tabular}
\end{table*}

\begin{table*}[t]
  \label{dataset2-table2}
  \centering \small
  \begin{tabular}{lllll}
    \toprule
    Dataset & Objects & Features & Classes & $CH_{A}$ \\
    \midrule

        Parkinsons & 195 & 22 & 2 & 0.033 \\ % Parkinsons Disease Dataset
    HTRU2 & 17,898 & 8 & 2 & 0.033 \\ % Pulsar Dataset HTRU2
        Siberian Weather Stats & 1,439 & 11 & 9 & 0.030 \\
        Patient Treatment Classification & 4,412 & 10 & 2 & 0.029 \\
        SMS Spam Collection & 835 & 500 & 2 & 0.027 \\ % sms
        MAGIC Gamma Telescope & 19,020 & 10 & 2 & 0.027 \\
        Orbit Classification For Prediction / NASA & 1,748 & 11 & 6 & 0.024 \\ % Orbit NASA 
         \midrule
        \midrule
        Harberman's Survival & 306 & 3 & 2 & 0.024 \\
        IMDB & 3,250 & 700 & 2 & 0.022 \\ % imdb
        Pumpkin Seeds  & 2,500 & 12 & 2 & 0.022 \\
        World12d & 150 & 12 & 5 & 0.021 \\
        Heart Attack Analysis \& Prediction & 303 & 13 & 2 & 0.021 \\
        Diabetic Retinopathy Debrecen & 1,151 & 19 & 2 & 0.020 \\
        Seismic Bumps & 646 & 24 & 2 & 0.017 \\ % seismic
        Hepatitis & 80 & 19 & 2 & 0.017 \\
        Statlog (German Credit) & 1,000 & 24 & 2 & 0.014 \\ % German Credit Numeric
        Wine Quality & 4,898 & 11 & 7 & 0.013 \\
        Sentiment Labeled Sentences & 2,748 & 200 & 2 & 0.013 \\ % sentiment
        Pima Indians Diabetes Database & 768 & 8 & 2 & 0.013 \\
        Blood Transfusion Service Center & 748 & 4 & 2 & 0.013 \\
        Heart Disease & 297 & 13 & 5 & 0.012 \\
        Cardiovascular Study & 2,927 & 15 & 2 & 0.011 \\
        Insurance Company Benchmark  & 5,822 & 85 & 2 & 0.010 \\ % The Insurance Company (TIC) Benchmark
        Street View House Numbers & 732 & 1,024 & 10 & 0.008 \\ % svhn
        SkillCraft1 Master Table Dataset & 3,338 & 18 & 7 & 0.006 \\ % SkillCraft-StarCraft
        HIVA & 3,076 & 1,617 & 2 & 0.006 \\ % hiva
        Spambase & 4,601 & 57 & 2 & 0.005 \\
        Wilt & 4,339 & 5 & 2 & 0.005 \\
        Breast Cancer Coimbra & 116 & 9 & 2 & 0.005 \\
        SECOM & 1,567 & 590 & 2 & 0.005 \\ % secom
        Customer Classification & 1,000 & 11 & 4 & 0.003 \\
        Credit Risk Classification & 976 & 11 & 2 & 0.003 \\
        Planning Relax & 182 & 12 & 2 & 0.002 \\
        Taiwanese Bankruptcy Prediction & 6,819 & 95 & 2 & 0.002 \\ % Company Bankruptcy Prediction
        Labeled Faces in the Wild & 2,200 & 5,828 & 2 & 0.002 \\
        Water Quality & 2,011 & 9 & 2 & 0.001 \\
        Epileptic Seizure Recognition & 5,750 & 178 & 5 & 0.001 \\ % epileptic
        Paris Housing Classification & 10,000 & 17 & 2 & 0.000 \\
        Fraud Detection Bank  & 20,468 & 112 & 2 & 0.000 \\
        
    \bottomrule
    
  \end{tabular}
  
\end{table*}

\vfill

\end{document}
